# Supplementary material for: An Information Bottleneck Approach for Markov Model Construction
Source: arXiv:2404.02856 source file (2024-06-10)
Supplement: Supplementary file 1 [file SPIB_MSM_SI.pdf]

---

# Supplementary Information: An Information Bottleneck Approach for Markov Model Construction

---

Dedi Wang, Yunrui Qiu, Eric R. Beyerle,  
Xuhui Huang and Pratyush Tiwary

## I. SUPPLEMENTARY METHODS

---

### Algorithm 1 Update representative inputs

---

**Input:** a long unbiased trajectory  $\{\mathbf{X}^n\}$ , a set of state labels  $\{\mathbf{y}^n\}$ , SPIB model parameters  $\theta$

- 1: Map all the input samples to the learned bottleneck variables  $\{\mathbf{z}^n = \mu_\theta(\mathbf{X}^n)\}$
  - 2:  $K \leftarrow$  the number of non-empty states in  $\{\mathbf{y}^n\}$
  - 3: **for**  $i$  from 0 to  $K$  **do**
  - 4:      $\mathbf{z}_c^i \leftarrow$  calculate the center of each non-empty metastable state
  - 5:      $\mathbf{z}_{\text{rep}}^i \leftarrow$  identify the nearest sample for each center  $\mathbf{z}_c^i$  using Euclidean distance
  - 6: **end for**
  - 7: Return the new representative-inputs  $\{\mathbf{X}_{\text{rep}}^k = \mu_\theta^{-1}(\mathbf{z}_{\text{rep}}^i)\}_{k=1}^K$
- 

---

### Algorithm 2 SPIB

---

**Input:** a long unbiased trajectory  $\{\mathbf{X}^n\}$ , a set of initial state labels  $\{\mathbf{y}^n\}$ , RC dimensionality  $d$ , time delay  $\Delta t$ , tolerance  $tol$  and patience  $n_{\text{patience}}$  for stopping criteria, number of refinements

$n_{\text{refinements}}$

- 1: Randomly pick up one sample from each initial state as our initial representative-inputs  $\{\mathbf{X}_{\text{rep}}^k\}_{k=1}^K$  where the number of representative-inputs  $K$  is equal to the number of initial states
  - 2: Set  $\text{loss}_0, \text{loss}_1 \leftarrow 0$
  - 3: **for**  $i$  from 0 to  $n_{\text{refinements}} - 1$  **do**
  - 4:     **repeat**
  - 5:         Set  $\text{loss}_0 = \text{loss}_1$
  - 6:         Sample a minibatch  $\{\mathbf{X}^n\}$  and  $\{\mathbf{y}^n\}$
  - 7:          $\text{loss}_1 \leftarrow$  calculate the objective function  $\mathcal{L}$
  - 8:         Update the neural network parameters  $\theta$  including weights  $\{\omega_k\}_{k=1}^K$
  - 9:     **until**  $|\text{loss}_0 - \text{loss}_1| < tol$  for  $n_{\text{patience}}$  iterations
  - 10:     Update the state labels  $\{\mathbf{y}^n\}$  via  $\hat{\mathbf{y}}^n = \underset{i}{\operatorname{argmax}} \mathcal{D}_i(\mu(\mathbf{X}^n); \Delta t, \theta)$
  - 11:     Update the representative-inputs  $\{\mathbf{X}_{\text{rep}}^k\}_{k=1}^K$  via Algorithm 1
  - 12: **end for**
-

## A. Model hyperparameters

In this subsection, we employ a 10-fold cross-validation scheme to identify an optimized set of hyperparameters for different models, aiming to strike a balance between model complexities and the ability to generalize to new data. We also investigate the sensitivity of the kinetic models, constructed using tICA-KMeans, PCA-Kmeans, VAMPnets, and SPIB, to their respective model hyperparameters.

### 1. *tICA-KMeans*

For tICA-KMeans based MSMs, Supplementary Figure 1 summarizes the results of the scoring for Trp-cage. Supplementary Figure 2 shows the results of the scoring for HP35. Supplementary Figure 3 shows the results of the scoring for WW-domain. The set of optimized hyperparameters of tICA-KMeans based MSMs are summarized in Table 1.

Supplementary Table 1: Optimum tICA-KMeans hyperparameters

|           | lag time | $n_{\text{components}}$ | K   |
|-----------|----------|-------------------------|-----|
| Trp-cage  | 40 ns    | 3                       | 200 |
| HP35      | 25 ns    | 4                       | 200 |
| WW-domain | 40 ns    | 6                       | 100 |

### 2. *PCA-KMeans*

For PCA-KMeans based MSMs, Supplementary Figure 4 summarizes the results of the scoring for Trp-cage. Supplementary Figure 5 shows the results of the scoring for HP35. Supplementary Figure 6 shows the results of the scoring for WW-domain. The set of optimized hyperparameters of PCA-KMeans based MSMs are summarized in Table 2.

Supplementary Table 2: Optimum PCA-KMeans hyperparameters

|           | $n_{\text{components}}$ | K   |
|-----------|-------------------------|-----|
| Trp-cage  | 10                      | 100 |
| HP35      | 10                      | 100 |
| WW-domain | 20                      | 500 |

### 3. *VAMPnets*

In this study, VAMPnets are instantiated by fully connected neural networks featuring two hidden layers with rectified linear units (ReLUs) as the activation function for all hidden layers. The selection of the number of neurons within the hidden layers and other training hyperparameters is guided by the optimization of validation GMRQ scores. While experimenting with architectures with more than 2 hidden layers, we observed no significant improvement. On the contrary, deep neural networks introduced instability when learning more than 10 states. Consequently, we opted for a two-hidden-layer configuration to maintain consistency with SPIB. In all of our implementations, we utilized the Softmax activation function in the output layer and selected the label for input conformations based on the highest probability output.

Supplementary Figure 7 summarizes the results of the scoring for Trp-cage. Supplementary Figure 8 shows the results of the scoring for HP35. Supplementary Figure 9 shows the results of the scoring for WW-domain. The set of optimized hyperparameters of VAMPnets are summarized in Table 3.

Supplementary Table 3: Optimum VAMPnets hyperparameters

|           | lag time | NN | batch<br>size | lr     | epochs |
|-----------|----------|----|---------------|--------|--------|
| Trp-cage  | 40 ns    | 32 | 2048          | 0.01   | 10     |
| HP35      | 20 ns    | 32 | 1024          | 0.003  | 10     |
| WW-domain | 20 ns    | 64 | 2048          | 0.0001 | 20     |

### 4. *SPIB*

In this work, both the encoder and decoder of SPIB are nonlinear and parameterized by fully connected neural networks with two hidden layers. A rectified linear unit (ReLU) is used as the activation function for all hidden layers. The choice of the number of neurons within the hidden layers in the encoder and decoder, as well as other training hyperparameters, is determined based on optimizing the validation GMRQ scores. In all SPIB-based MSMs, we consistently employed the Softmax output with the highest probability to label the input conformations.

Our recommended tuning process involves fixing a large lag time  $\Delta t$  to derive a small number of macrostates and then sequentially tuning the other hyperparameters. Supplementary Figure 10 summarizes the results of the scoring for Trp-cage, where we fix  $\Delta t = 100$  ns. Supplementary Figure 11 shows the results of the scoring for HP35, with a fixed lag time of  $\Delta t = 100$  ns. Supplementary Figure 12 shows the results of the scoring for WW-domain, with a fixed lag time of  $\Delta t = 70$  ns. An optimal set of hyperparameters of SPIB, based on the highest test set GMRQ over a set of 10-fold cross validated models after conditionally scanning over the hyperparameter space as defined, are summarized in Table 4.

For a clearer understanding of the training process, a pseudo-code outlining the SPIB training procedure is presented in Algorithm 2.

Supplementary Table 4: Optimum SPIB hyperparameters

|          | tol  | $n_{\text{patience}}$ | N1 | N2 | batch<br>size | lr   | $d_z$ | $\beta$ | $n_{\text{refinements}}$ |
|----------|------|-----------------------|----|----|---------------|------|-------|---------|--------------------------|
| Trp-cage | 2e-3 | 2                     | 64 | 64 | 4096          | 3e-5 | 2     | 1e-3    | 15                       |
| HP35     | 1e-3 | 2                     | 64 | 64 | 4096          | 1e-5 | 2     | 3e-3    | 15                       |
| WWdomain | 5e-3 | 2                     | 32 | 32 | 4096          | 1e-3 | 2     | 1e-1    | 15                       |

## B. Coarse-graining into macrostates using PCCA+ and MPP

In this work, we use the deeptime software package<sup>1</sup> to perform the PCCA+ clustering and code from Gerhard Stock’s group<sup>2</sup> to perform the MPP clustering. To ensure that the MPP method yields the same number of states as obtained by SPIB, for Trp-cage system, we set  $Q_{\min} = 0.28$  and  $Q_{\min} = 0.15$  to obtain approximately 4 states and 10 states for tICA+K-Means and  $Q_{\min} = 0.22$  and  $Q_{\min} = 0.13$  to obtain approximately 4 states and 10 states for PCA+K-Means, respectively. For HP35, we set  $Q_{\min} = 0.5$  and  $Q_{\min} = 0.2$  to obtain about 5 states and 10 states for tICA-MPP based MSM and  $Q_{\min} = 0.222$  and  $Q_{\min} = 0.1$  to obtain approximately 5 states and 10 states for PCA-MPP based MSM, respectively. Similarly, for the WW-domain, we set  $Q_{\min} = 0.44$  and  $Q_{\min} = 0.19$  to obtain approximately 5 states and 10 states for tICA-MPP based MSM and  $Q_{\min} = 0.13$  and  $Q_{\min} = 0.07$  to obtain approximately 4 states and 10 states for PCA-MPP based MSM. To ensure MPP can capture states with small populations, we set a minimum population

threshold of 0.1%.

### C. Effect of training hyperparameters and initial state labels for SPIB

SPIB demonstrates robustness across a wide spectrum of hyperparameter values, illustrated in Supplementary Figure 10 (Trp-cage), Supplementary Figure 11 (HP35), and Supplementary Figure 12 (WW-domain). Despite reporting a specific set of parameters in Table 4, the main point of this set of supplementary information is the robustness of the SPIB method to hyperparameter selection, and, for the protein trajectories studied here, the learned models are stable within the displayed hyperparameter ranges. Thus, slightly different sets of hyperparameters than those reported in Table 4 can be used to generate effective SPIB models for studying protein folding dynamics.

Here we test the effect of different initial state labeling schemes on the performance of SPIB constructed MSMs. Supplementary Figure 13 shows how the initial labels generated by different hyperparameters of tICA-KMeans will affect the SPIB in constructing macrostate models, with the GMRQ score used as the quality-measurement metric. To further test the performance of different initial state scheme, we also test the implementation of PCA-KMeans to generate the initial state labels as shown in Supplementary Figure 16. Similar results are demonstrated for the HP35 protein in Supplementary Figure 14 (tICA-KMeans) and Supplementary Figure 17 (PCA-KMeans). The WW-domain protein exhibits analogous results in Figure 15 (tICA-KMeans) and Figure 18 (PCA-KMeans). All the robustness tests mentioned above were conducted by training SPIB with a large time delay  $\Delta t$ .

We extended the robustness tests to include various quality-measurement metrics (i.e. GMRQ score, metastability, shannon entropy and DBI) using two distinct time delays  $\Delta t$ . For a large time delay, we observe robustness in the results with the choice of the initial label schemes. Both tICA+kmeans and PCA+kmeans initial state labels yield the same states. Supplementary Figure 19 shows the effect of different initial state label scheme in Trp-cage. Similar results are also shown in Supplementary Figure 20 for HP35 and Supplementary Figure 21 for WW-domain.

However, with a moderate time delay, these two schemes may result in different intermediate states and consequently, slightly different outcomes. Since the time delay  $\Delta t$  for SPIB remains fixed, the resulting number of macrostates may vary depending on different initial

labels, leading to some comparisons being less equitable. Supplementary Figure 22 shows the effect of different initial state label scheme in Trp-cage. Similar results are also shown in Supplementary Figure 23 for HP35 and Supplementary Figure 24 for WW-domain. As a general recommendation, we suggest using tICA+kmeans for improved capture of slow dynamics, leading to better GMRQ and metastability. On the other hand, PCA+kmeans is preferred for learning more structurally distinct states, enhancing the DBI. Additionally, it is important to note that when using PCA+kmeans for generating initial labels, it typically requires the inclusion of more principal components compared to schemes based on tICA.

All results in the main text are derived using tICA+kmeans for generating initial state labels. Given SPIB’s robustness to the hyperparameters of tICA-KMeans, we employ the optimal tICA-KMeans hyperparameters, selected based on validation GMRQ scores and outlined in Supplementary Table 1, for generating initial state labels.

## II. SUPPLEMENTARY RESULTS

### A. Trp-Cage

#### 1. *Quantitative comparison*

Supplementary Figure 25 shows the Trp-cage quantitative results for 4-state model, and Supplementary Figure 26 shows the Trp-cage quantitative results for 10-state model in terms of GMRQ, metastability, Shannon entropy, and DBI. Supplementary Figure 27 shows the implied timescales for 4-state model and Supplementary Figure 28 shows the implied timescales for 10-state model. Supplementary Figure 29 shows the CK test performed for both 4-state model and 10-state model at 100 ns lag time. For the 10-state model, we find the residence probability of state 0 decays to 0 for long lag time. This outcome is attributed to the state’s small population, accounting for only 0.002%, and the constraints posed by limited sampling.

#### 2. *Qualitative comparison*

With a large time delay  $\Delta t = 100$  ns, Supplementary Figure 30 visually represents the state partitioning among macrostates obtained from various methods. SPIB demonstrates

a high degree of consistency with VAMPnets in capturing similar microstates (Supplementary Figure 30(e)). However, both tICA-PCCA+ (Supplementary Figure 30(c)) and PCA-PCCA+ (Supplementary Figure 30(d)) successfully identify the same states but struggle to precisely delineate the boundary between state 0 and state 1 as identified by SPIB. In contrast, PCA-MPP exhibits challenges in discriminating between state 0 and state 1 of SPIB (Supplementary Figure 30(b)). Furthermore, tICA-MPP fails to differentiate state 0, state 1, and state 2 of SPIB (Supplementary Figure 30(a)), instead erroneously learning two sparsely populated states (state 2 and state 3 identified by tICA-MPP).

We assess the influence of utilizing different methods for macrostate construction by comparing them to the reference method SPIB in the context of learning a 10-state model with a moderate time delay  $\Delta t = 10$  ns in Supplementary Figure 31. Clearly, with a smaller time delay  $\Delta t$ , SPIB is able to learn a finer grained model with more macrostates where the majority of macrostates are well populated. This behavior is in contrast to the other methods as shown in Supplementary Figure 32, where these methods generally fail to further divide those highly populated states, resulting in many lowly populated states. Performing MPP and PCCA+ on PCA seems able to alleviate the problem, but they generally fail to perform well in dynamical metrics.

From Supplementary Figure 31, the major difference between the macrostates from SPIB and macrostates from other methods is that other methods generally fail to have better resolution or divide the molten globule state with 73% population and the unfolded state consisting of multiple turns with 7.5% population. See the structure visualization in the main text.

## B. HP35

### 1. *Quantitative comparison*

Supplementary Figure 33 shows the HP35 quantitative results for 5-state models constructed with , and Supplementary Figure 34 shows the HP35 quantitative results for the 10-state model in terms of GMRQ, metastability, Shannon entropy, and DBI.

Supplementary Figure 35 shows the implied timescales for 5-state model and Supplementary Figure 36 shows the implied timescales for 10-state model. For the implied timescales

results, the 5-state SPIB model is constructed using a  $\Delta t = 110$  ns. Supplementary Figure 37 shows the CK test performed for the 5-state and 10-state models at 100 ns lag time. For the 5-state model, all learned metastable states obey the CK condition to a good approximation. The same is true for the 10-state model, with the exception of state 9, which shows a slight disagreement between the predicted and propagated probabilities at the longest lag time tested (500 ns). These results help support the claims made in the main text regarding the SPIB method’s ability to generate effective kinetic models at multiple temporal and spatial resolutions.

## 2. *Qualitative comparison*

With a large time delay  $\Delta t = 100$  ns, Supplementary Figure 38 visually represents the state partitioning among macrostates obtained from the methods used to generate metastable states examined in the main text. SPIB demonstrates a high degree of consistency with tICA + MPP in capturing similar macrostates (Supplementary Figure 38(a)). For the other methods (PCA + MPP, Supplementary Figure 38b; tICA + PCCA+, Supplementary Figure 38c; PCA + PCCA+, Supplementary Figure 38d; VAMPnet, Supplementary Figure 38e) the two most populated folded states differing in the  $\phi_3$  dihedral angle are collapsed into a single state. All methods identify roughly the same ‘hub’ state with  $\alpha_2$  and  $\alpha_3$  folded but  $\alpha_1$  unfolded described in the main text, with the differences coming from the other unfolded and misfolded states less metastable than the two folded states and the hub unfolded state. Using a 10 state model for the other metastable clustering approaches enhances their abilities to distinguish the two folded states, as shown in Supplementary Figures 39 and 40, where the two folded states are allocated their own metastable states for every method sampled.

It is possible that the differences in metastable clustering for both the 5 and 10 state models affect the predicted folding mechanism in a model-dependent manner, but we did not examine this difference in any detail as an intricate analysis of differential model-dependent folding mechanisms are beyond the scope of this work.

## C. WW domain

### 1. *Quantitative comparison*

Supplementary Figure 41 shows the WW domain quantitative results for 5-state model, and Supplementary Figure 42 shows the WW domain quantitative results for 10-state model in terms of GMRQ, metastability, Shannon entropy, and DBI. Supplementary Figure 43 shows the implied timescales for 5-state model and Supplementary Figure 44 shows the implied timescales for 10-state model. Supplementary Figure 45 shows the CK test performed for both 5-state model and 10-state model constructed by SPIB at 100ns lag time. The consistency between SPIB-MSMs and MD simulations validates the predictive power of MSMs.

### 2. *Qualitative comparison*

The macrostates constructed by different methods are subsequently aligned and compared using the Sankey plot. With SPIB trained with a large time delay of  $\Delta t = 70$  ns as reference, Supplementary Figure 46 visualizes the relations between different 5-states models. Clearly, all methods except the PCA-MPP method successfully and consistently identified the folded, unfolded, and misfolded states. However, due to the low populations of partially-folded intermediate states, the boundaries of these states vary across different methods. Based on the ITS results, clear timescale separation is observed between the 2nd and 3rd eigenmodes, while other fast eigenmodes exhibit similar timescales. This observation demonstrates the clarity in identifying three metastable states, while other states may be mixed.

With SPIB trained with a large time delay of  $\Delta t = 10$  ns as reference, Supplementary Figure 47 visualizes the relations between different 10-states models. In general, SPIB results show greater consistency with tICA-PCCA+ and PCA-PCCA+ outcomes, whereas VAMP-net and MPP-based methods struggle to effectively separate the unfolded and partial-folded states. Additional structural information regarding SPIB macrostates can be found in the main text. Based on the results and comparisons, SPIB demonstrates significant capability in distinguishing meaningful intermediate states and concurrently categorizing folded and unfolded states based on different interactions between terminal residues. Moreover, the relationships between the 5-state and 10-state models constructed by the same method are

also visualized in Supplementary Figure 48.

## SUPPLEMENTARY REFERENCES

- <sup>1</sup>M. Hoffmann, M. Scherer, T. Hempel, A. Mardt, B. de Silva, B. E. Husic, S. Klus, H. Wu, N. Kutz, S. L. Brunton, and F. Noé, Machine Learning: Science and Technology **3**, 015009 (2021).
- <sup>2</sup>D. Nagel, “Moldyn freiburg,” <https://github.com/moldyn/Clustering> (2021), [Online; accessed 27-November-2023].

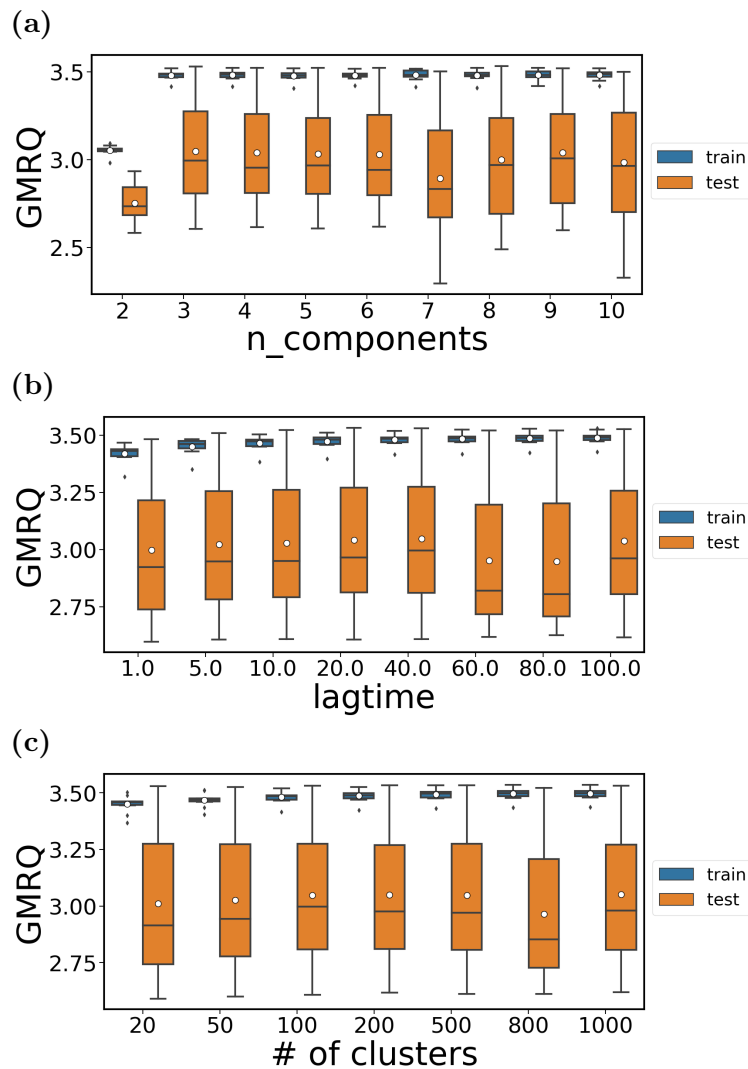

**Supplementary Figure 1:** Trp-cage 10-fold cross validation results for optimal hyperparameter choice for tICA-KMeans. The GMRQ scores are calculated using top 3 eigenvalues at a 100 ns lag time. The tICA lag time is measured in ns.

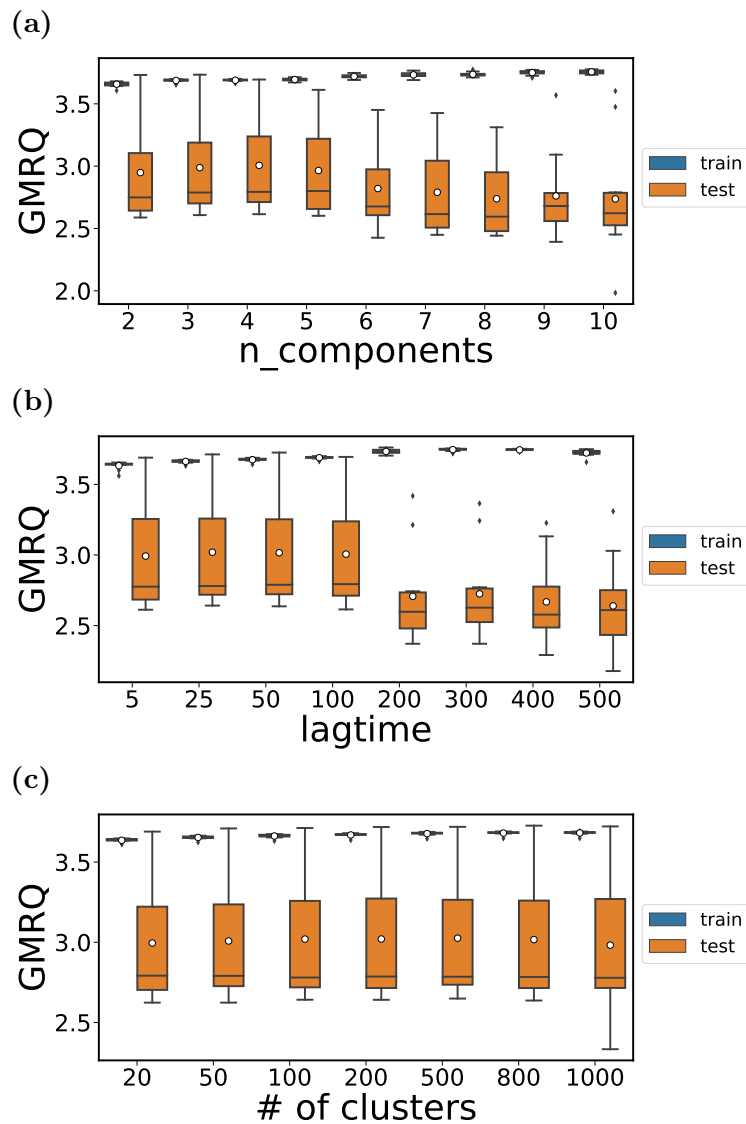

**Supplementary Figure 2:** HP35 10-fold cross validation results for optimal hyperparameter choice for tICA-KMeans. The GMRQ scores are calculated using top 3 eigenvalues at a 100 ns lag time. The tICA lag time is measured in ns.

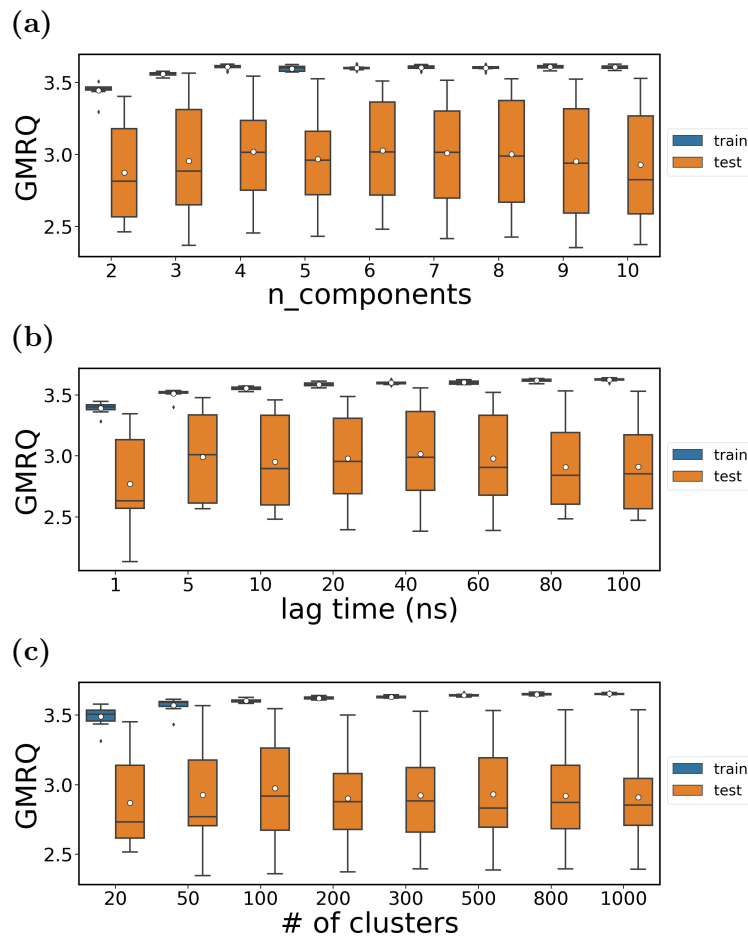

**Supplementary Figure 3:** WW-domain 10-fold cross validation results for optimal hyperparameter choice for tICA-KMeans. The GMRQ scores are calculated using top 3 eigenvalues at a 100 ns lag time. The tICA lag time is measured in ns.

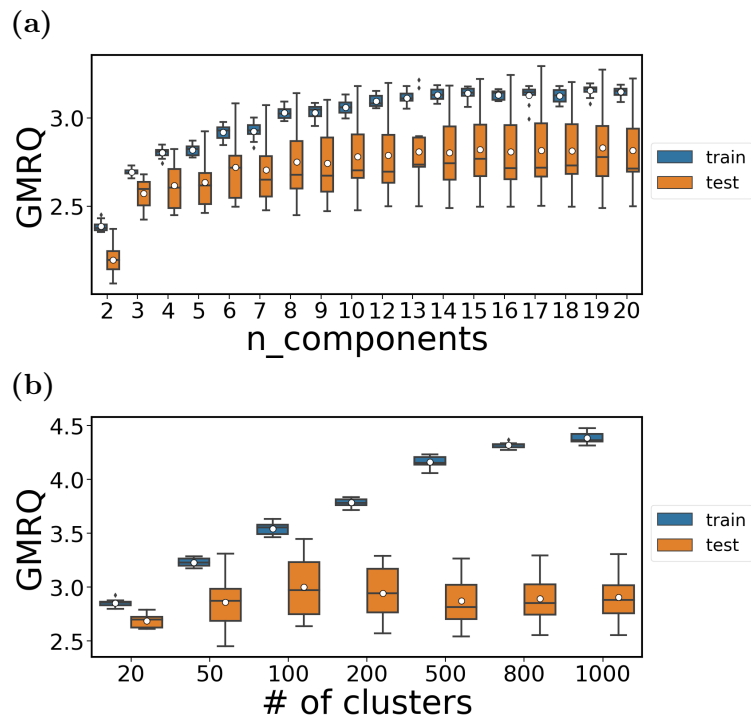

**Supplementary Figure 4:** Trp-cage 10-fold cross validation results for optimal hyperparameter choice for PCA-KMeans. The GMRQ scores are calculated using top 3 eigenvalues at a 100 ns lag time.

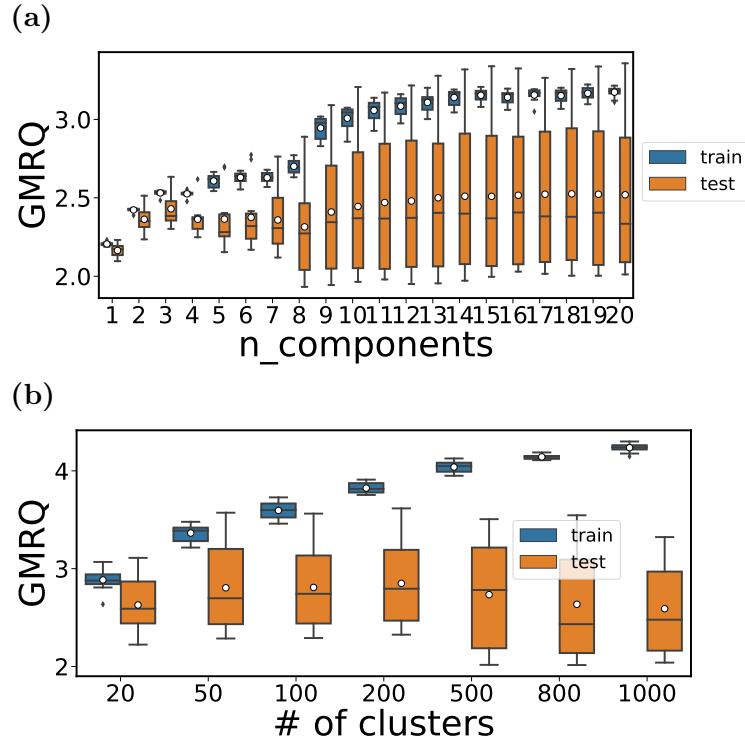

**Supplementary Figure 5:** HP35 10-fold cross validation results for optimal hyperparameter choice for PCA-KMeans. The GMRQ scores are calculated using top 3 eigenvalues at a 100 ns lag time.

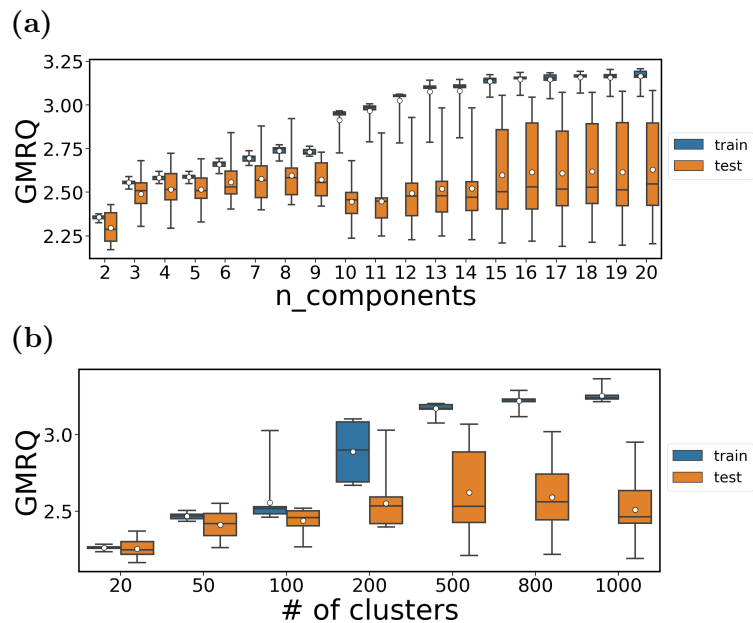

**Supplementary Figure 6:** WW-domain 10-fold cross validation results for optimal hyperparameter choice for PCA-KMeans. The GMRQ scores are calculated using top 3 eigenvalues at a 100 ns lag time.

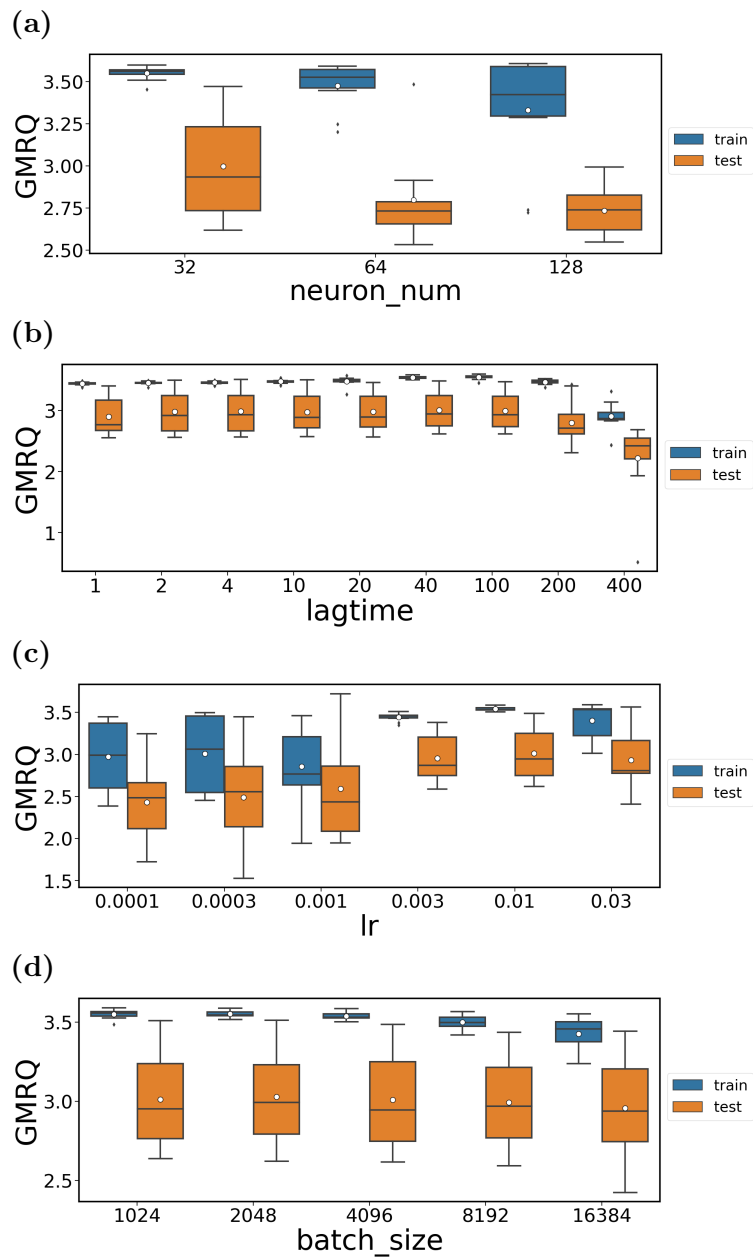

**Supplementary Figure 7:** Trp-cage 10-fold cross validation results for optimal hyperparameter choice for VAMPnets. The GMRQ scores are calculated using top 3 eigenvalues at a 100 ns lag time. The VAMPnet lag time is measured in ns.

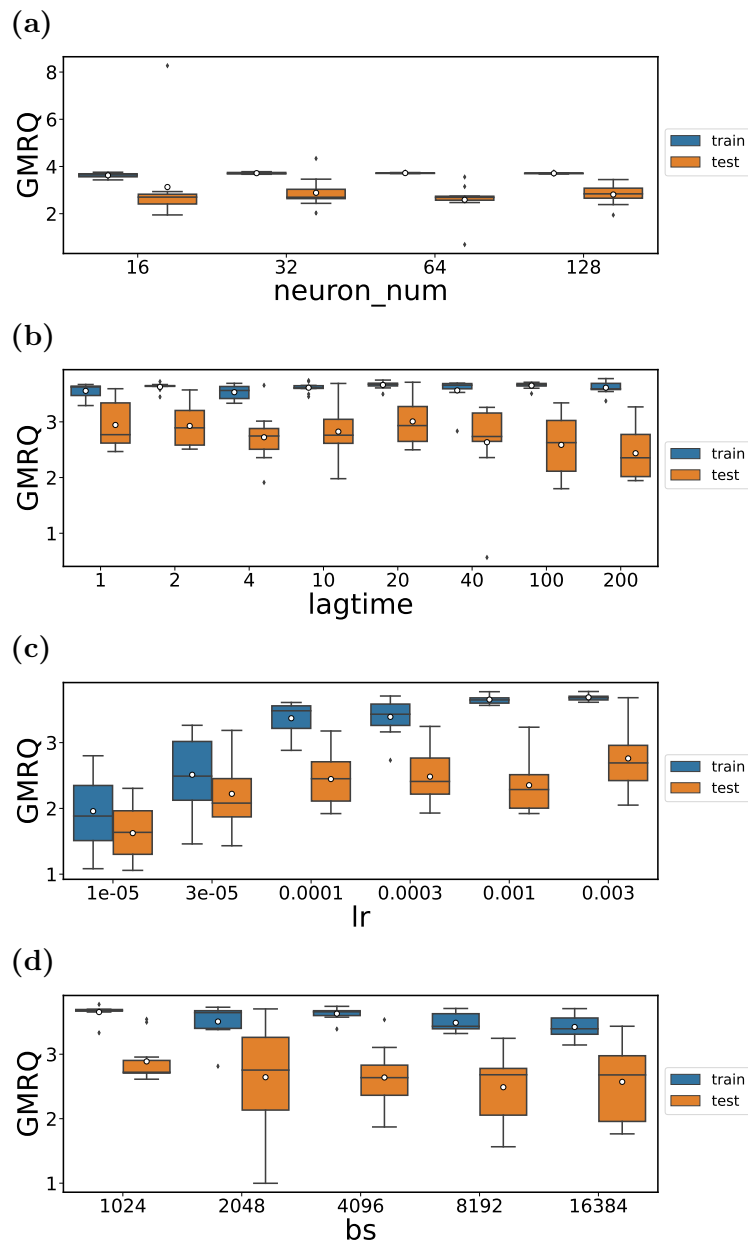

**Supplementary Figure 8:** HP35 10-fold cross validation results for optimal hyperparameter choice for VAMPnets. The GMQR scores are calculated using top 3 eigenvalues at a 100 ns lag time. The VAMPnet lag time is measured in ns.

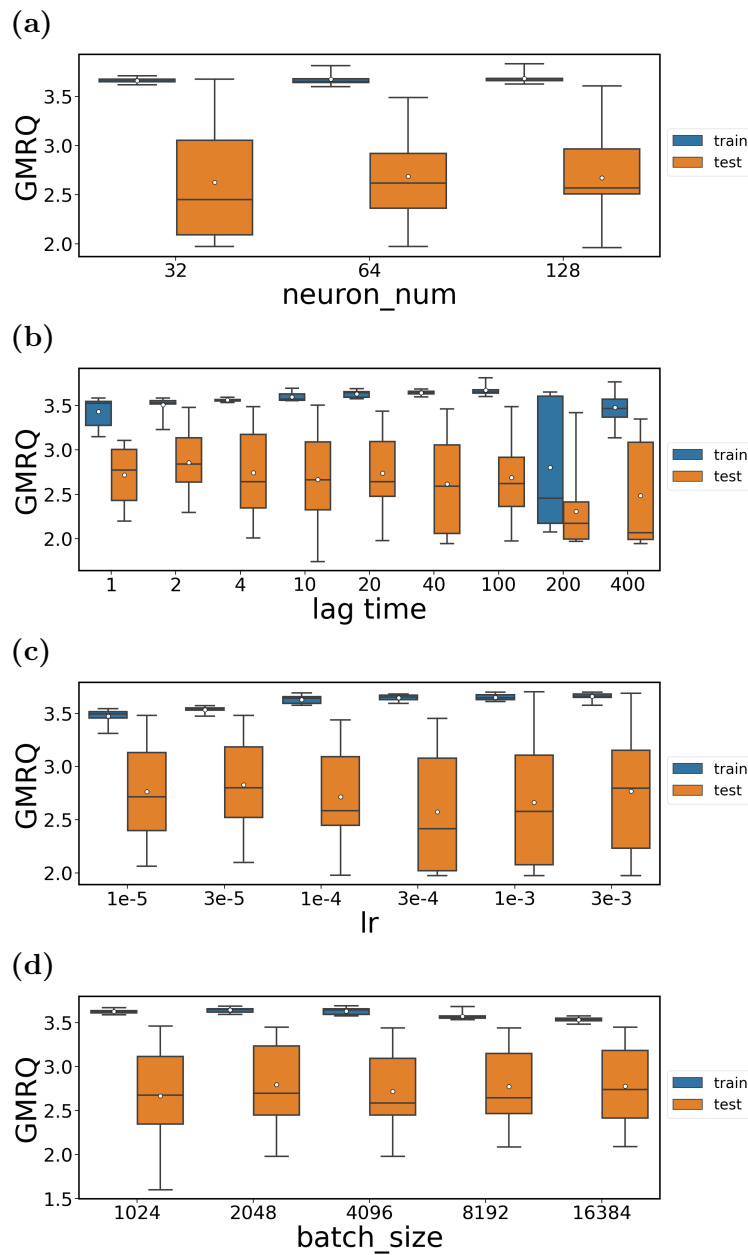

**Supplementary Figure 9:** WW-domain 10-fold cross validation results for optimal hyperparameter choice for VAMPnets. The GMRQ scores are calculated using top 3 eigenvalues at a 100 ns lag time. The VAMPnet lag time is measured in ns.

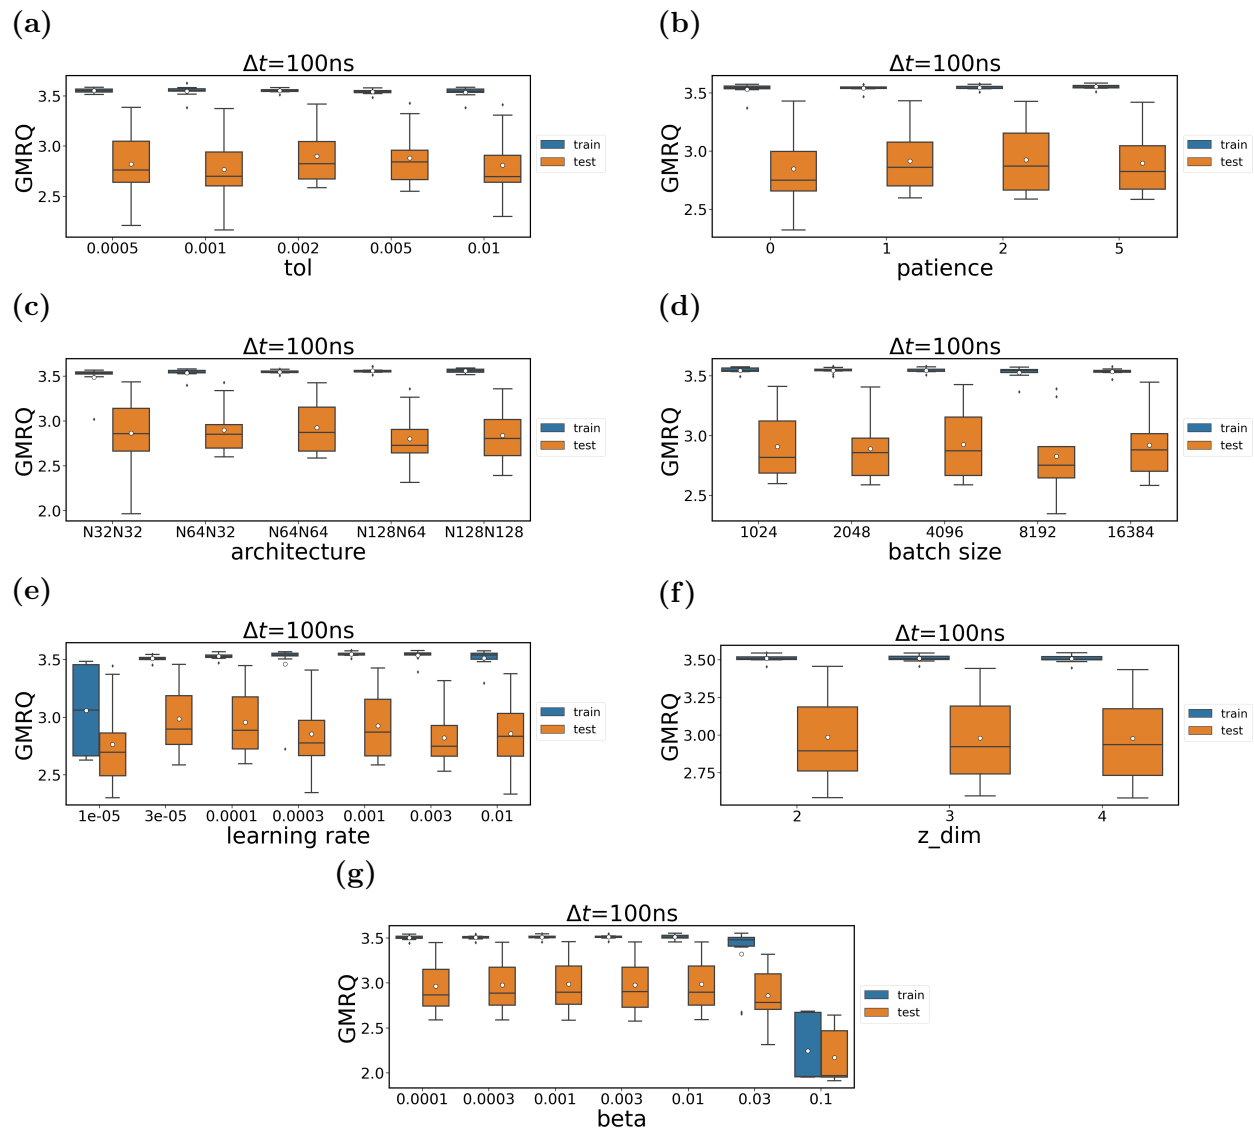

**Supplementary Figure 10:** Trp-cage 10-fold cross validation results for optimal hyperparameter choice for SPIB. The GMRQ scores are calculated using top 3 eigenvalues at a 100 ns lag time.

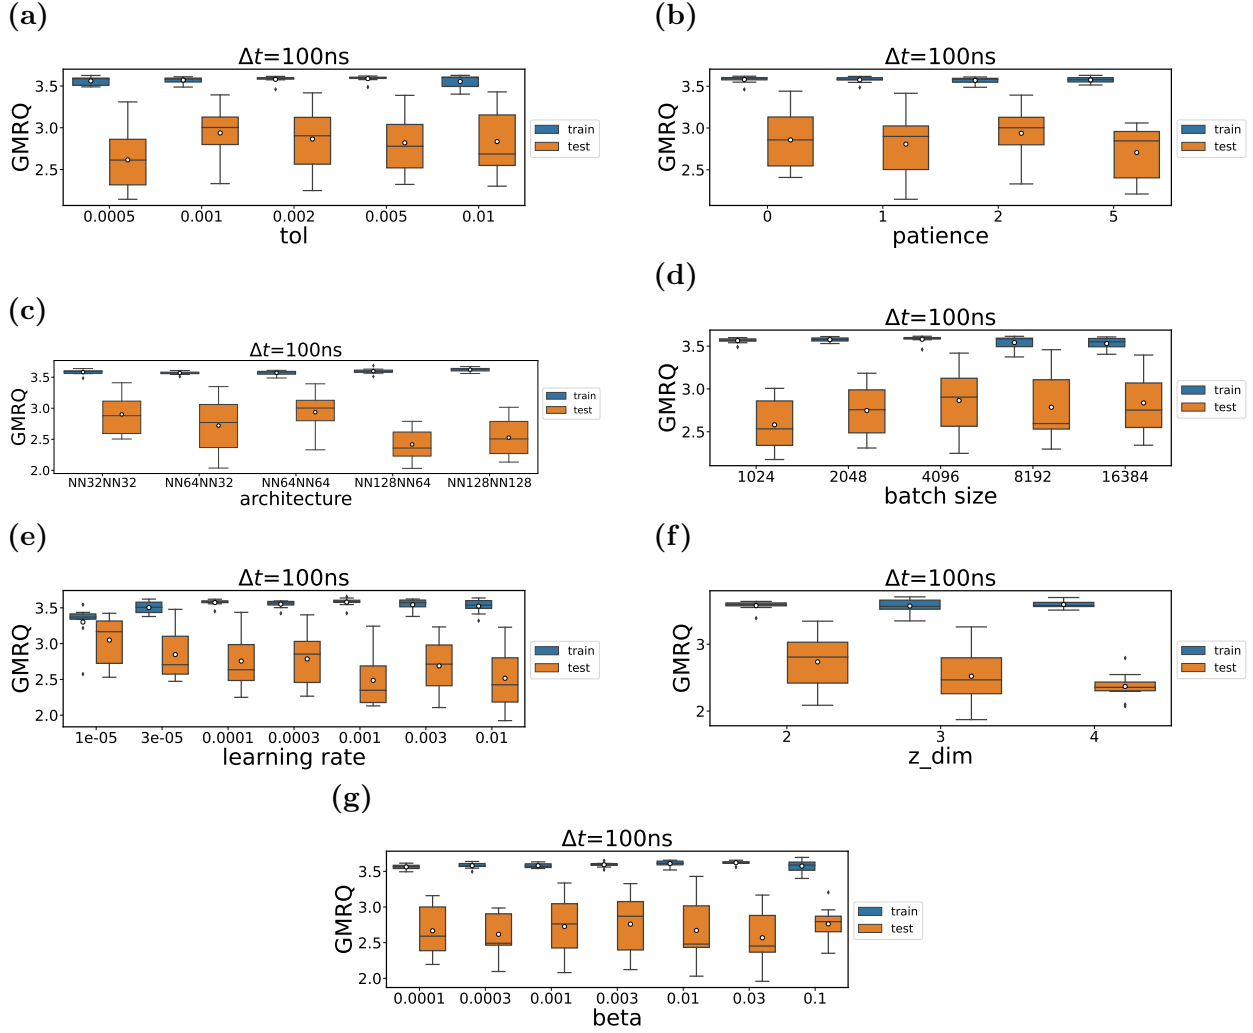

**Supplementary Figure 11:** HP35 10-fold cross validation results for optimal hyperparameter choice for SPIB. The GMRQ scores are calculated using top 3 eigenvalues at a 100 ns lag time.

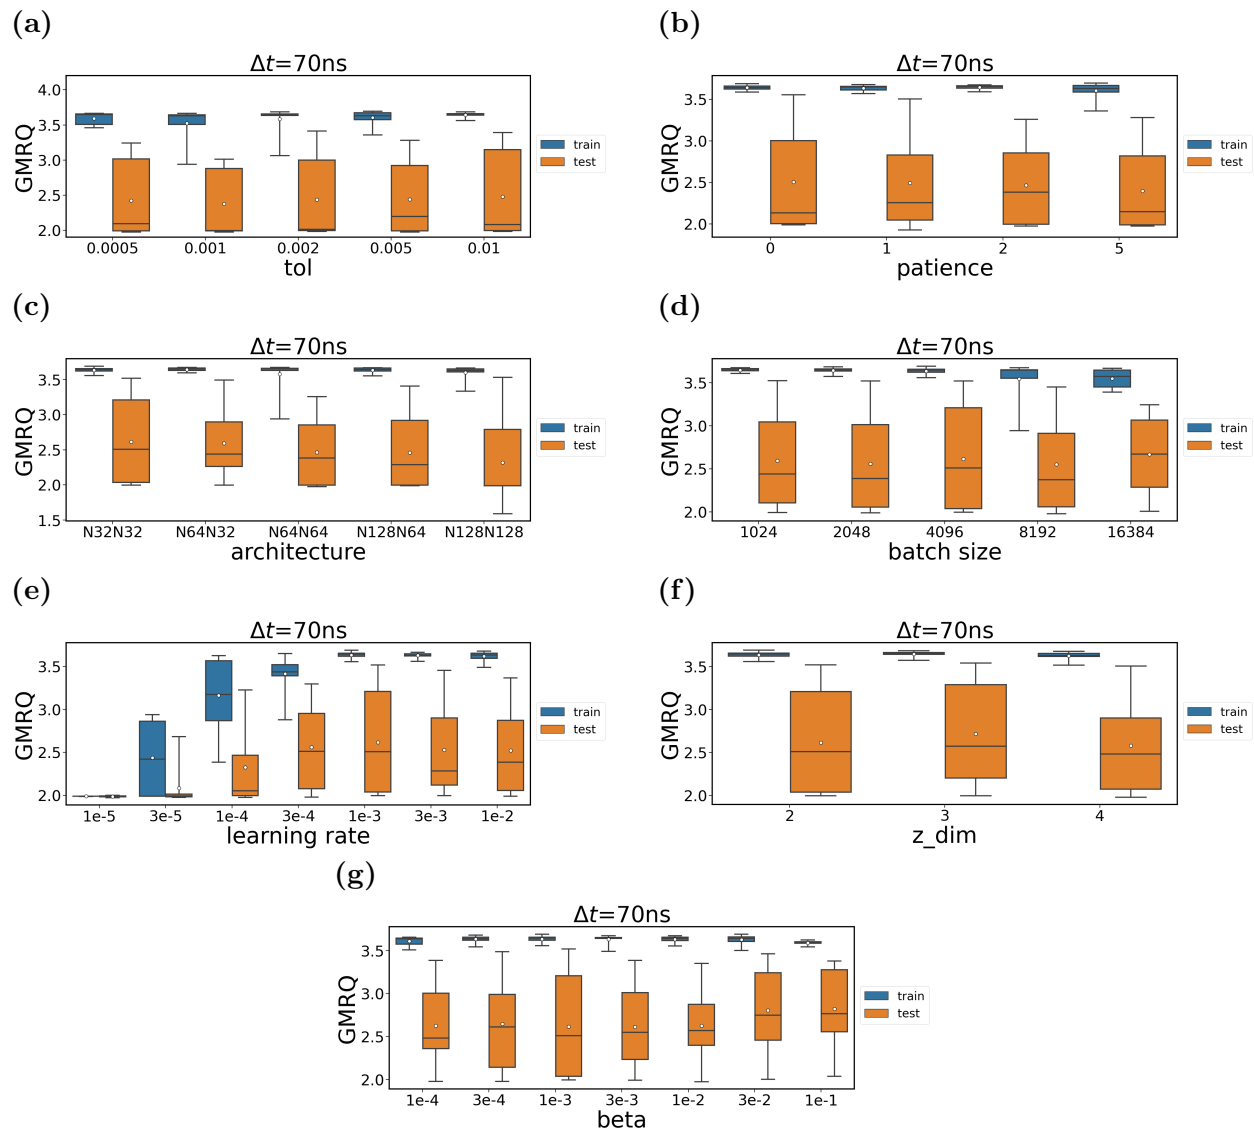

**Supplementary Figure 12:** WW-domain 10-fold cross validation results for optimal hyperparameter choice for SPIB. The GMRQ scores are calculated using top 3 eigenvalues at a 100 ns lag time.

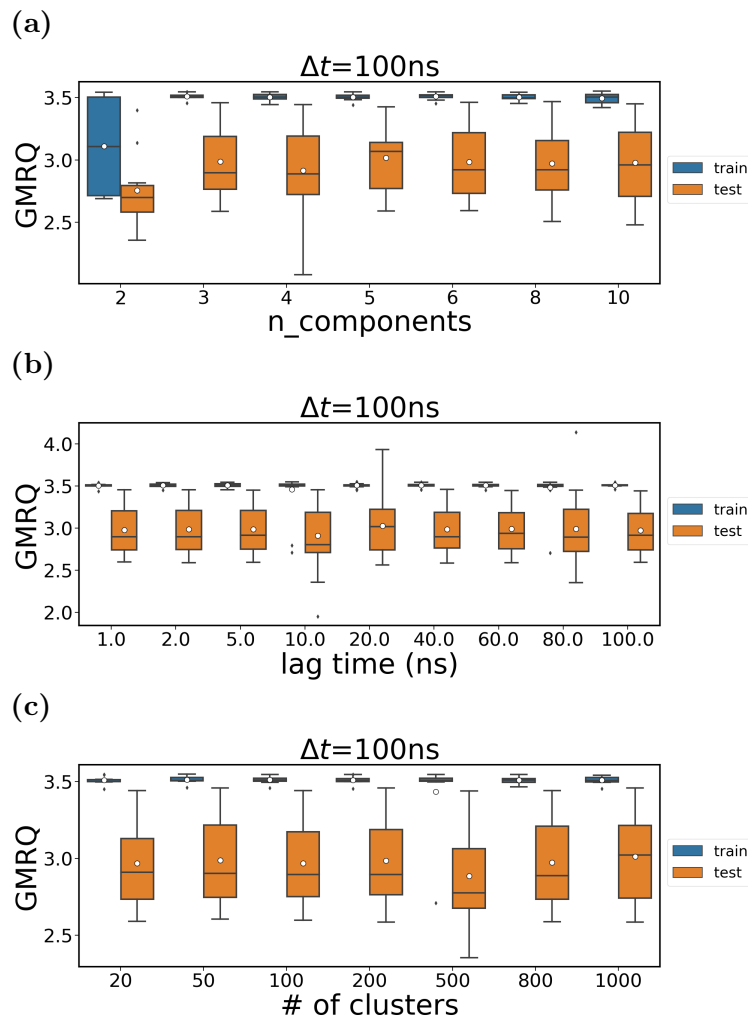

**Supplementary Figure 13:** Effect of the hyperparameters of tICA-KMeans on the initial state labels for Trp-cage. The GMRQ scores are calculated using top 3 eigenvalues at a 100 ns lag time.

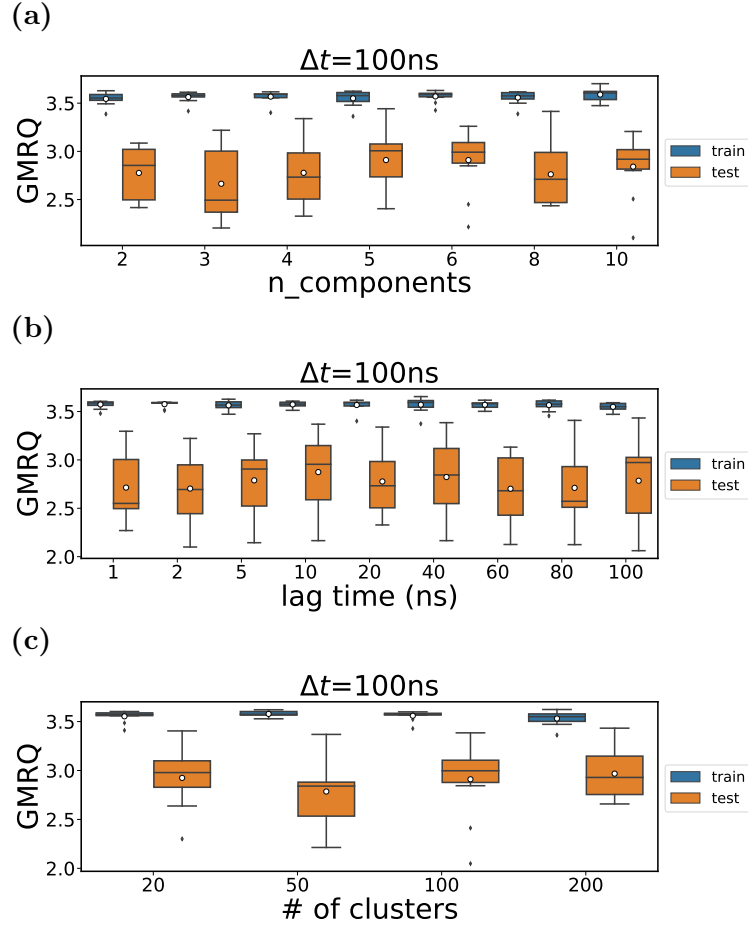

**Supplementary Figure 14:** Effect of the hyperparameters of tICA-KMeans on the initial state labels for HP35. The GMRQ scores are calculated using top 3 eigenvalues at a 100 ns lag time.

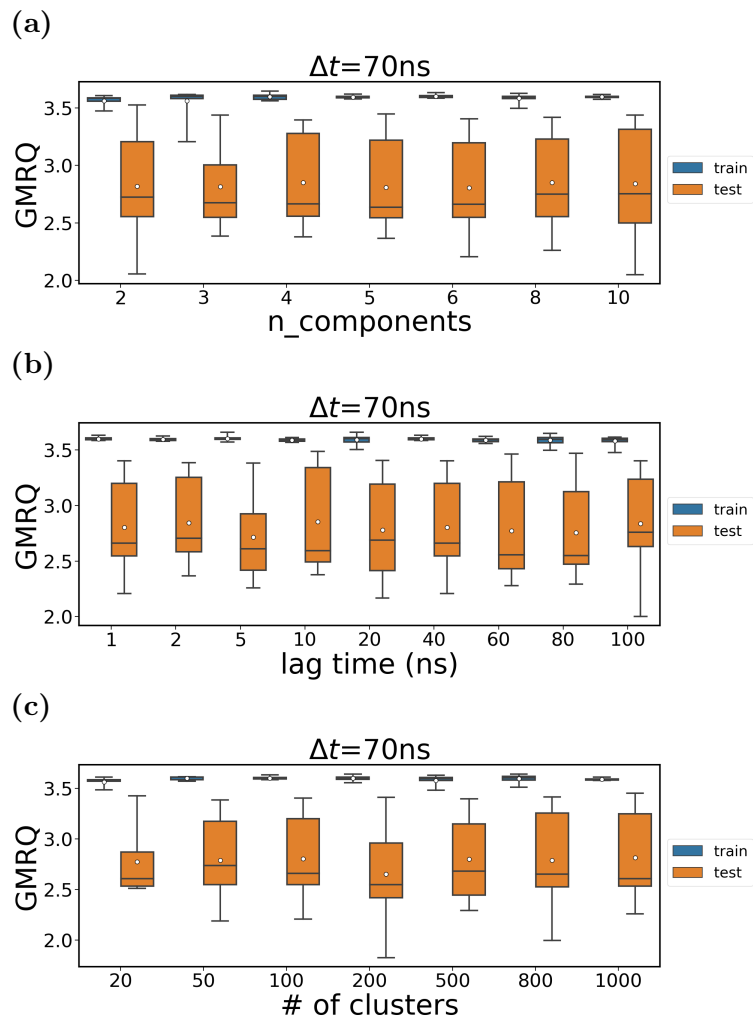

**Supplementary Figure 15:** Effect of the hyperparameters of tICA-KMeans on the initial state labels for WW-domain. The GMRQ scores are calculated using top 3 eigenvalues at a 100 ns lag time.

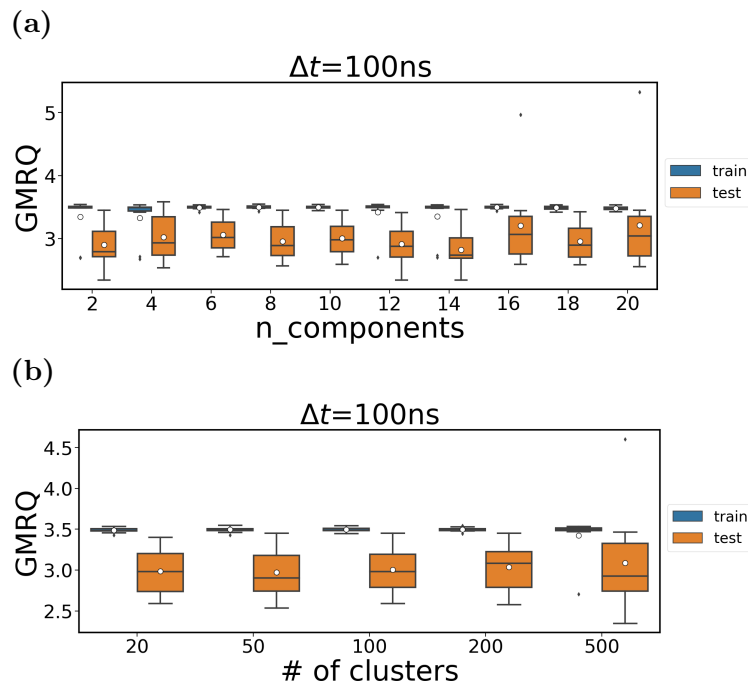

**Supplementary Figure 16:** Effect of the hyperparameters of PCA-KMeans on the initial state labels for Trp-cage. The GMRQ scores are calculated using top 3 eigenvalues at a 100 ns lag time.

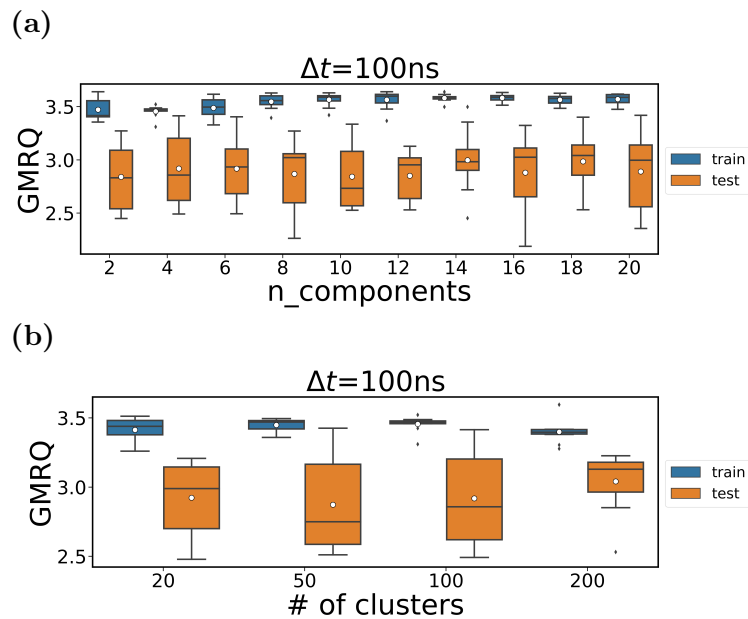

**Supplementary Figure 17:** Effect of the hyperparameters of PCA-KMeans on the initial state labels for HP35. The GMRQ scores are calculated using top 3 eigenvalues at a 100 ns lag time.

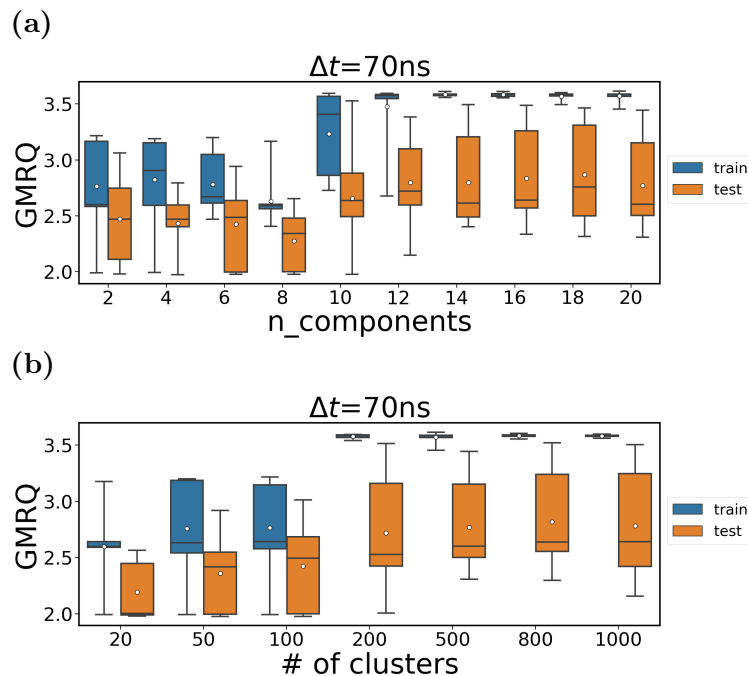

**Supplementary Figure 18:** Effect of the hyperparameters of PCA-KMeans on the initial state labels for WW-domain. The GMRQ scores are calculated using top 3 eigenvalues at a 100 ns lag time.

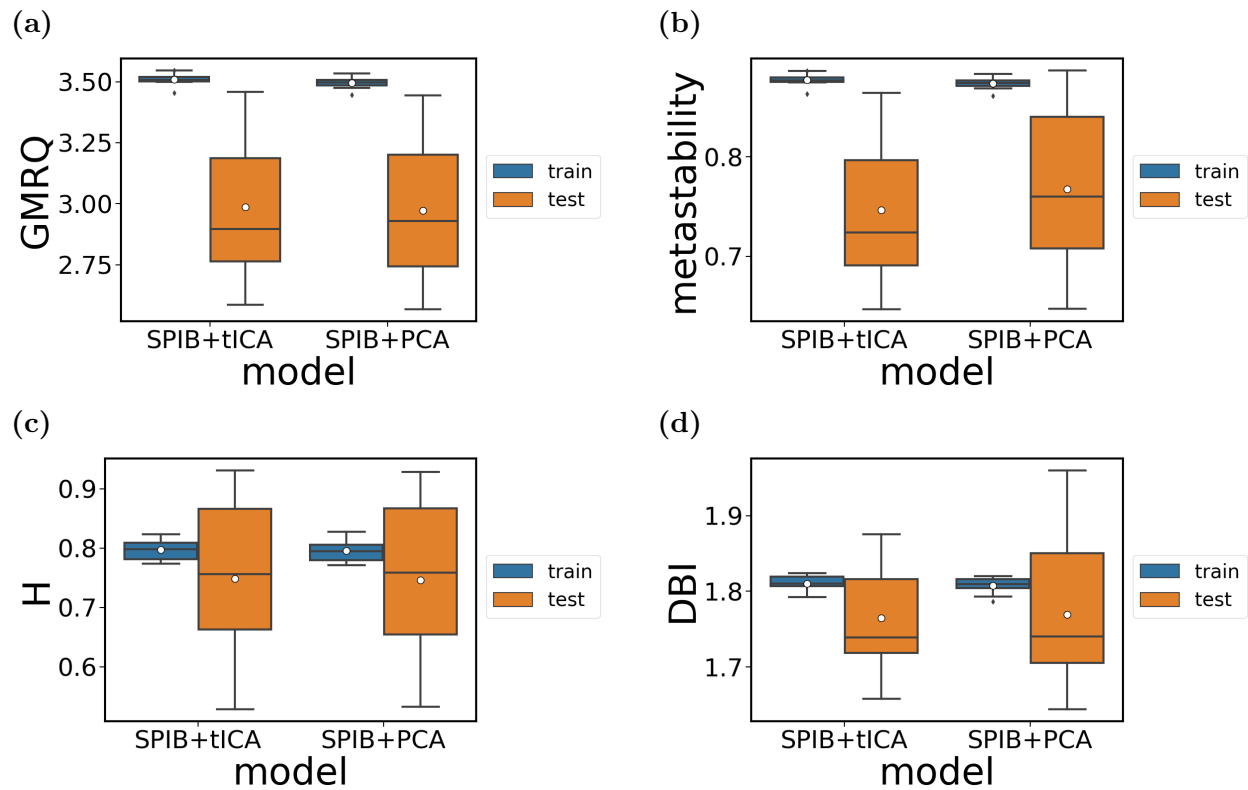

**Supplementary Figure 19:** Effect of initial state labels on Trp-cage results for  $\Delta t = 100$  ns. The GMRQ scores are calculated using top 3 eigenvalues at a 100 ns lag time.

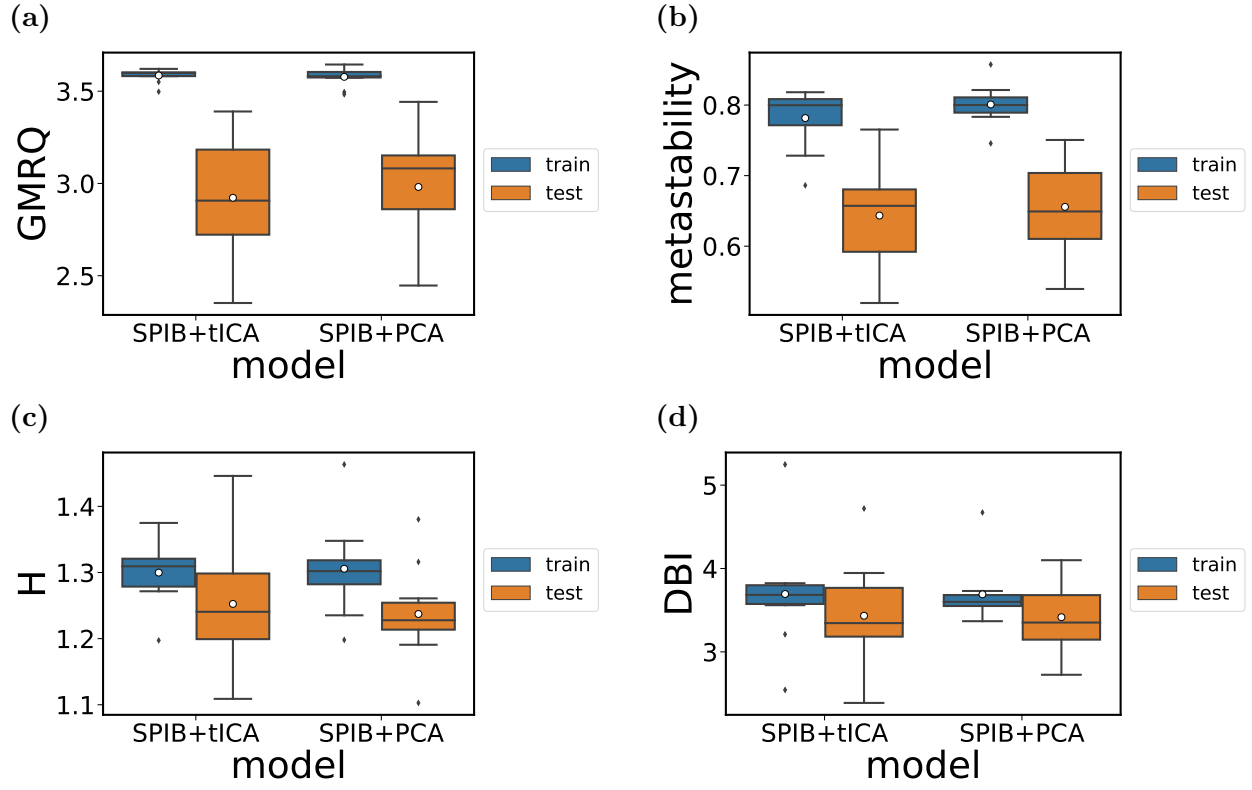

**Supplementary Figure 20:** Effect of initial state labels on HP35 results for  $\Delta t = 100$  ns. The GMRQ scores are calculated using top 3 eigenvalues at a 100 ns lag time.

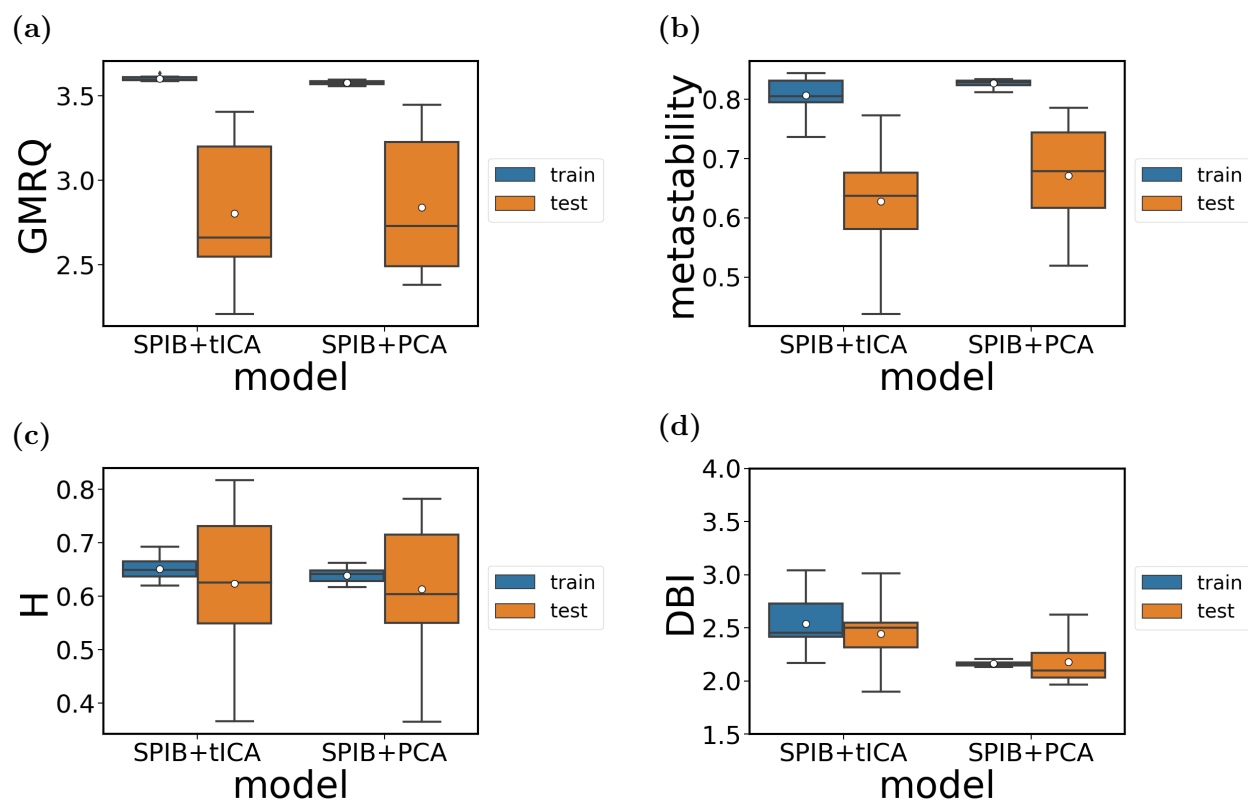

**Supplementary Figure 21:** Effect of initial state labels on WW-domain results for  $\Delta t = 70$  ns. The GMRQ scores are calculated using top 3 eigenvalues at a 100 ns lag time.

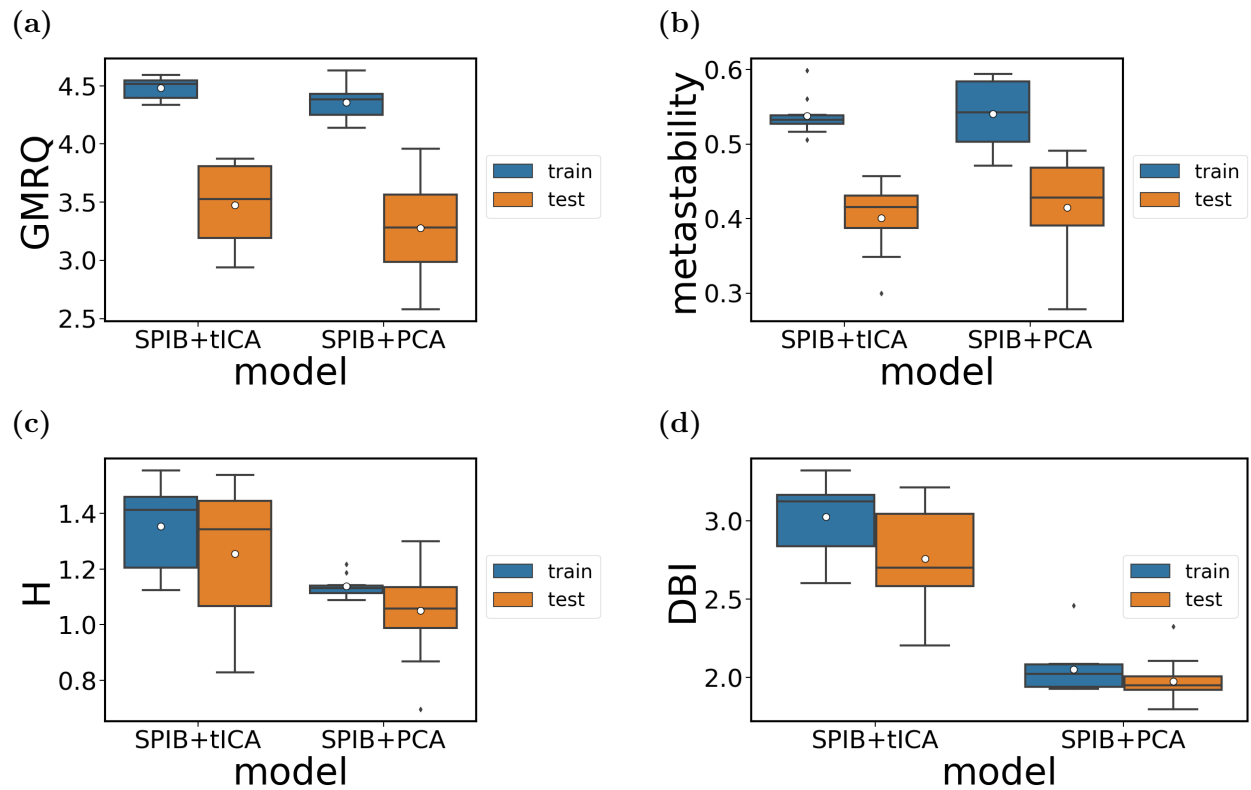

**Supplementary Figure 22:** Effect of initial state labels on Trp-cage results for  $\Delta t = 10$  ns. The GMRQ scores are calculated using top 3 eigenvalues at a 100 ns lag time.

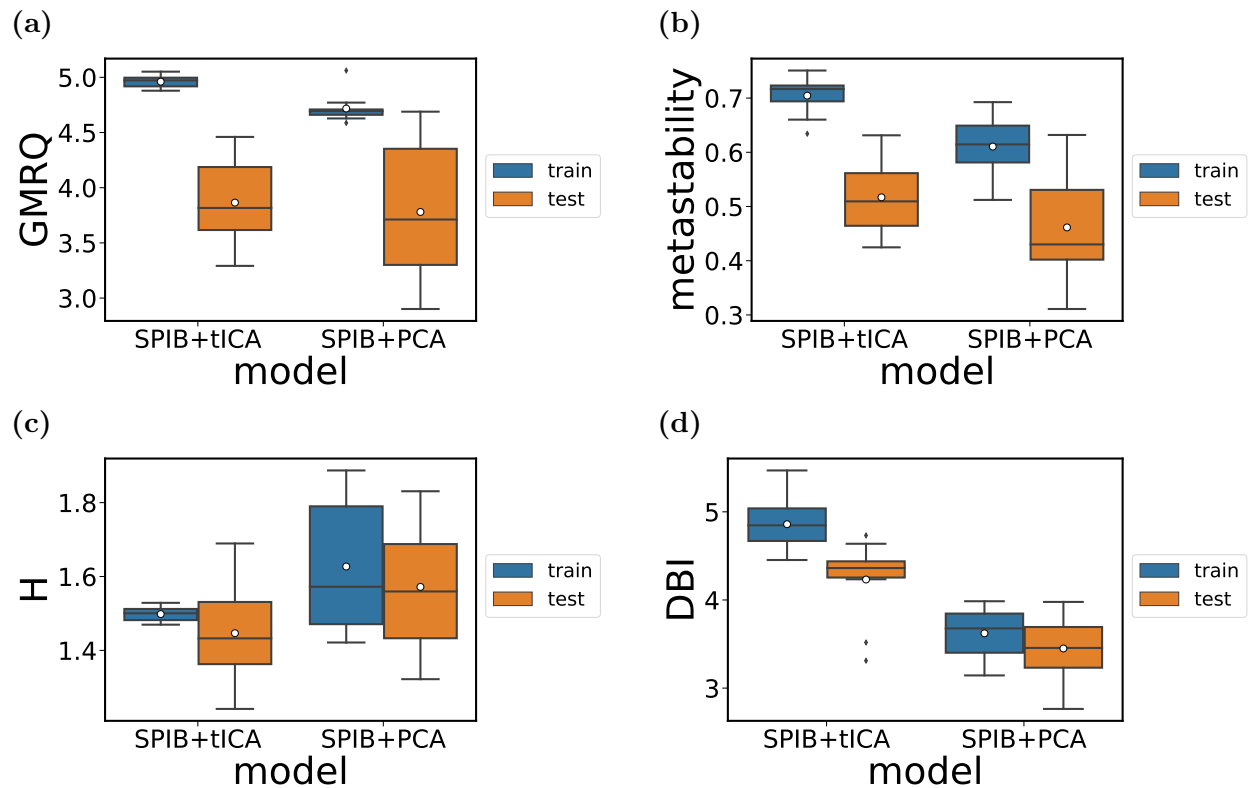

**Supplementary Figure 23:** Effect of initial state labels on HP35 results for  $\Delta t = 20$  ns. The GMRQ scores are calculated using top 5 eigenvalues at a 100 ns lag time.

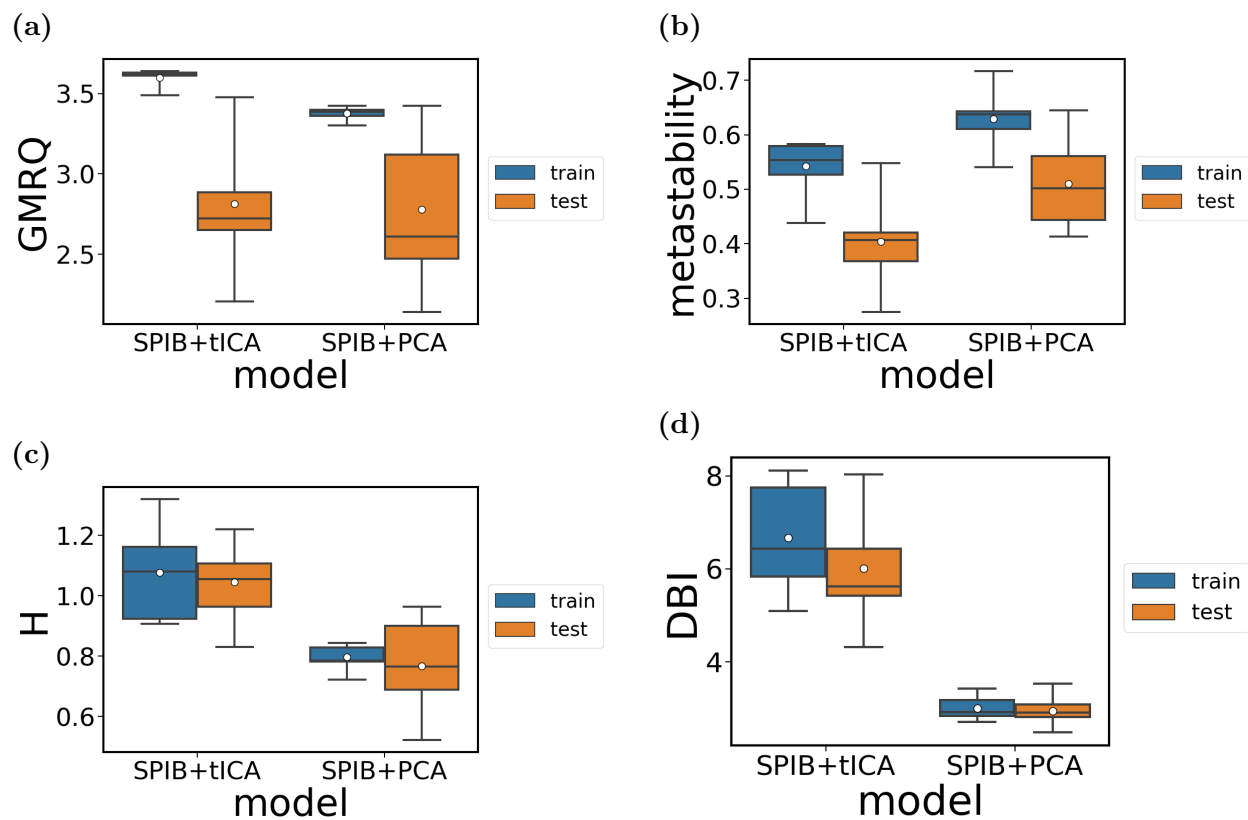

**Supplementary Figure 24:** Effect of initial state labels on WW-domain results for  $\Delta t = 10$  ns. The GMRQ scores are calculated using top 3 eigenvalues at a 100 ns lag time.

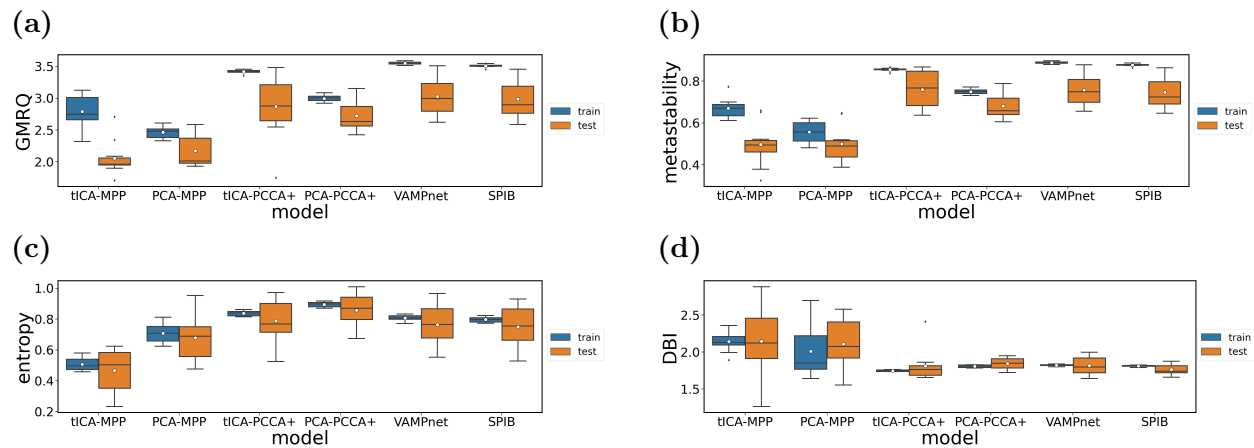

**Supplementary Figure 25:** Trp-cage quantitative results for 4-state model. The GMRQ scores are calculated using top 3 eigenvalues at a 100 ns lag time.

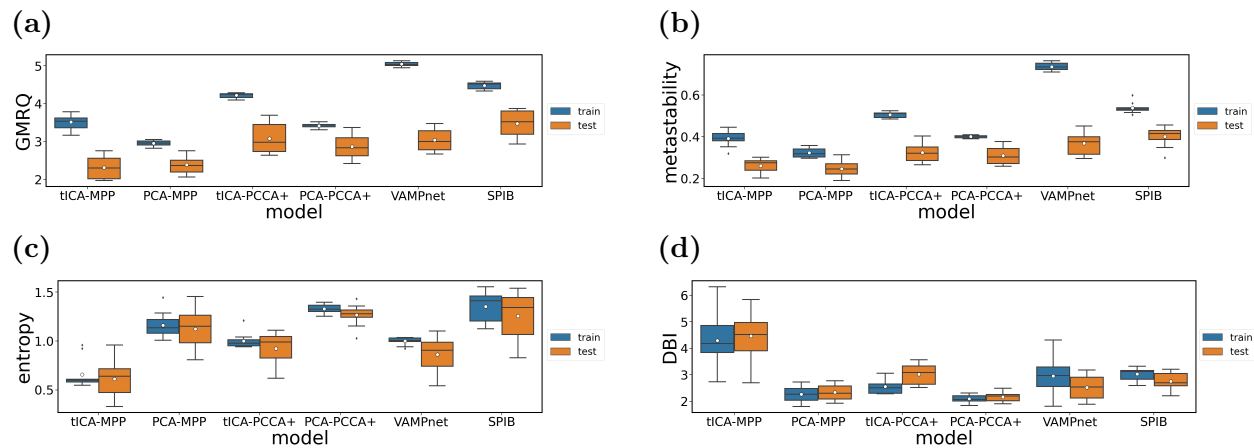

**Supplementary Figure 26:** Trp-cage quantitative results for 10-state model. The GMRQ scores are calculated using top 5 eigenvalues at a 100 ns lag time.

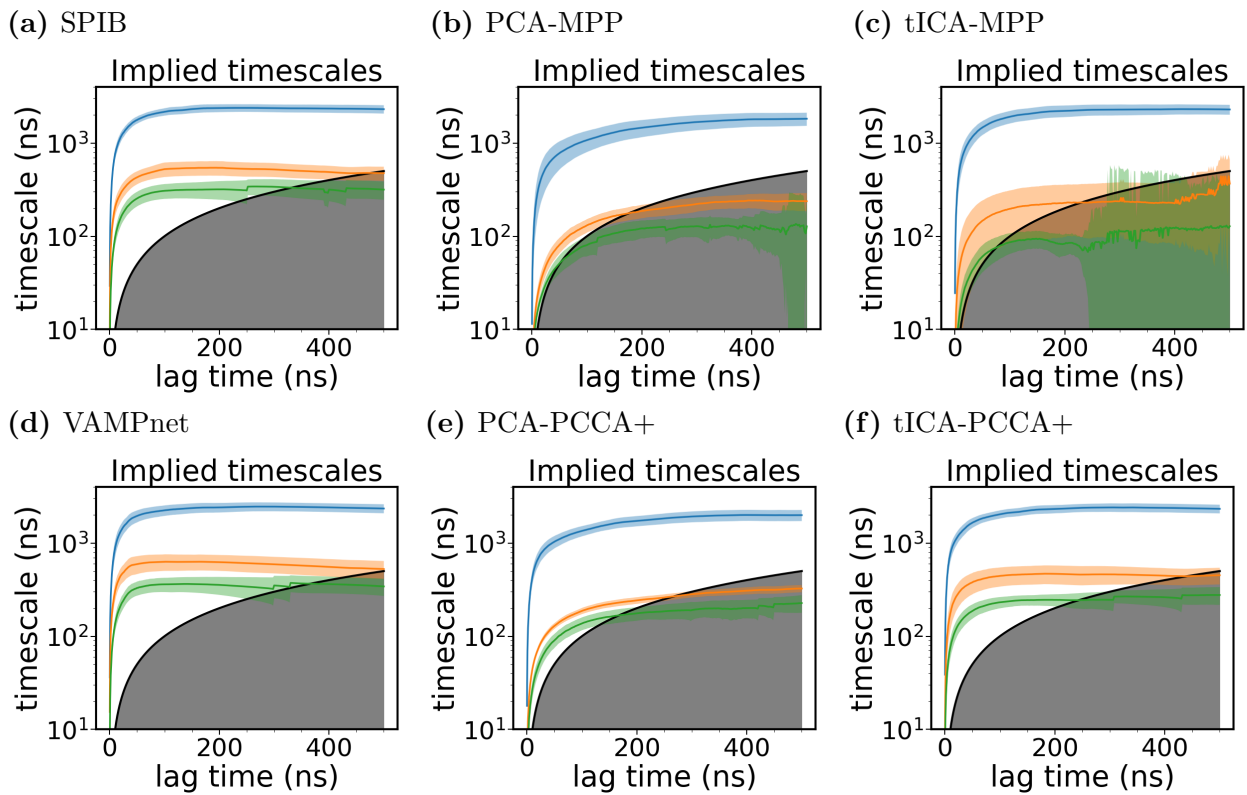

**Supplementary Figure 27:** Implied time scales as a function of lag time for the 4-state MSMs of Trp-cage. The shaded gray area represents the region where time scales become equal to or smaller than the lag time and can no longer be resolved. 95% confidence interval error bars are reported over 10 bootstrapping runs.

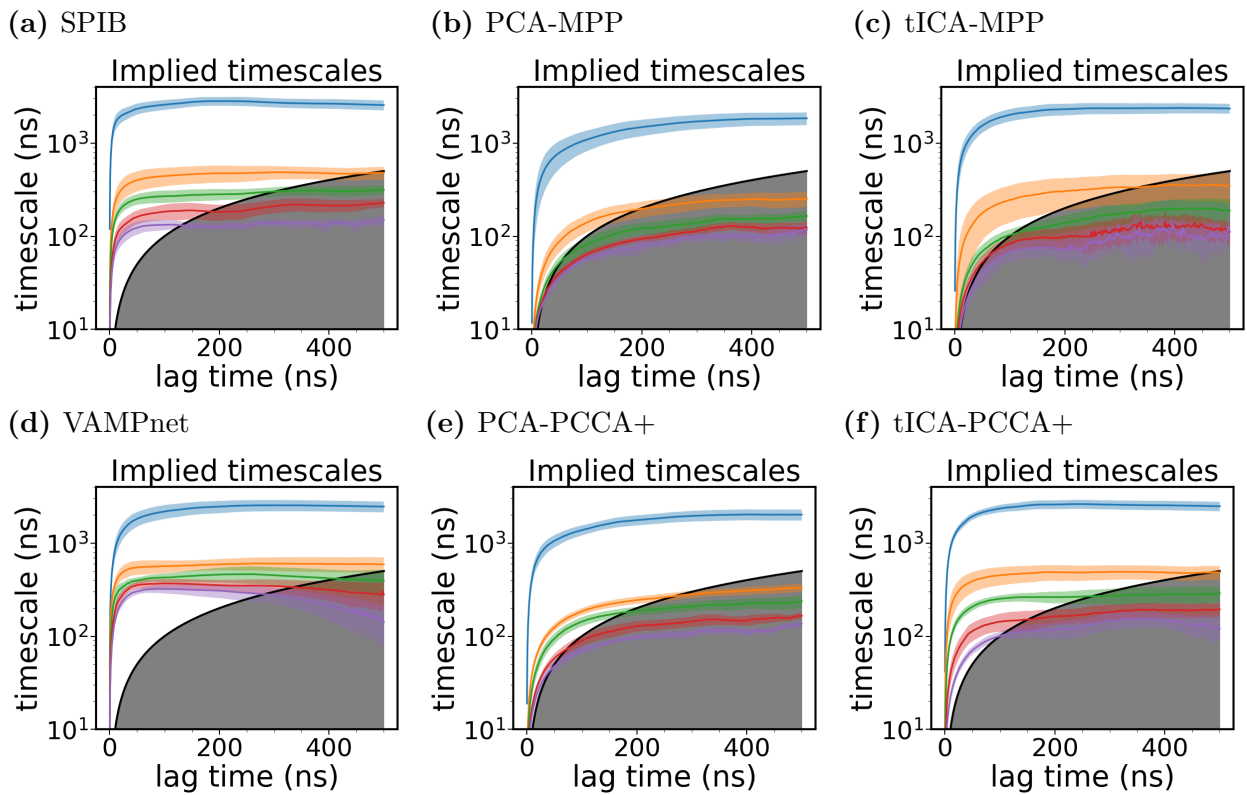

**Supplementary Figure 28:** Implied time scales as a function of lag time for the 10-state MSMs of Trp-cage. The shaded gray area represents the region where time scales become equal to or smaller than the lag time and can no longer be resolved. 95% confidence interval error bars are reported over 10 bootstrapping runs.

(a) 4-state

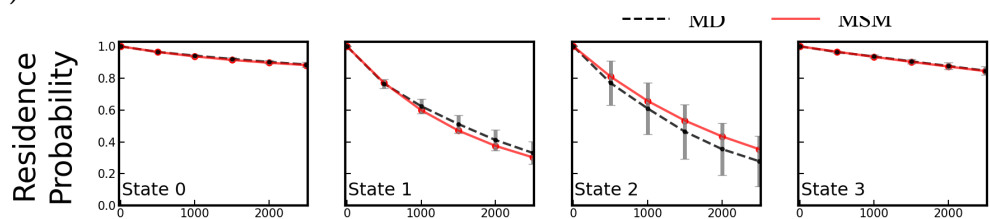

(b) 10-state

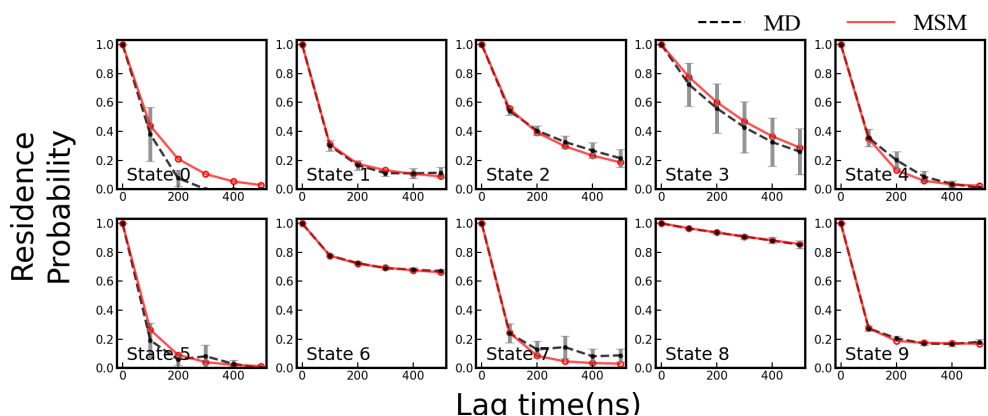

**Supplementary Figure 29:** The Chapman-Kolmogorov (CK) test utilizes residence probabilities for both the 4-macrostate (a) and 10-macrostate (b) MSMs constructed by SPIB for the Trp-cage folding system. The agreement between the residence probabilities predicted by 100ns SPIB-MSMs (solid red line) and those directly estimated from MD simulations (dashed black line) serves as validation for the MSMs. The error bar is estimated by bootstrapping MD trajectories 50 times with replacement.

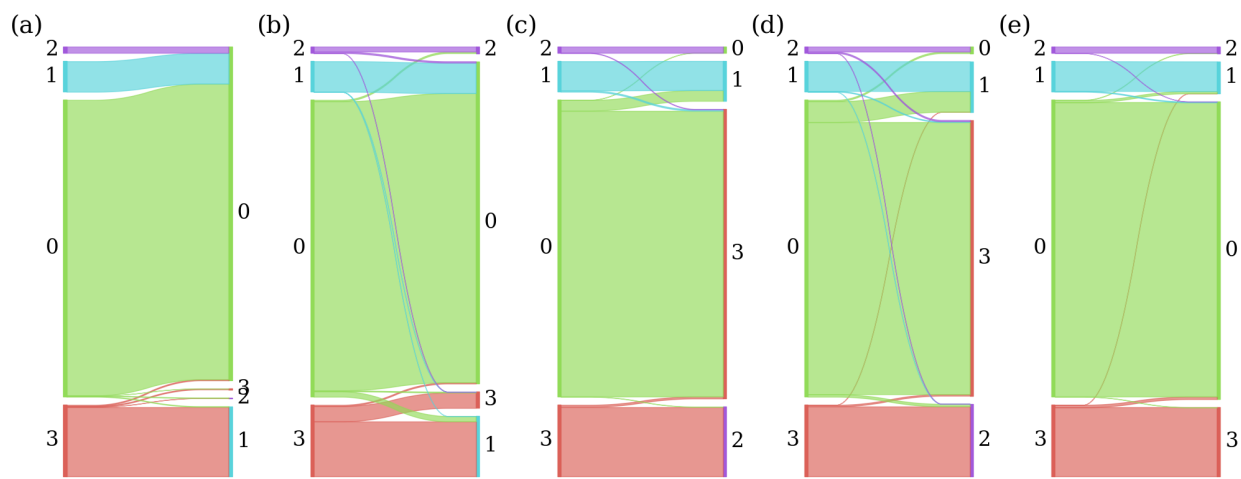

**Supplementary Figure 30:** The impact of employing alternative methods for macrostate construction is evaluated in comparison to the reference method SPIB for learning a 4-state model for Trp-cage. Each Sankey diagram illustrates the states obtained using SPIB (on the left) juxtaposed with states from alternative methods (on the right): (a) tICA-MPP model, (b) PCA-MPP model, (c) tICA-PCCA+ model, (d) PCA-PCCA+ model, and (e) VAMPnets model.

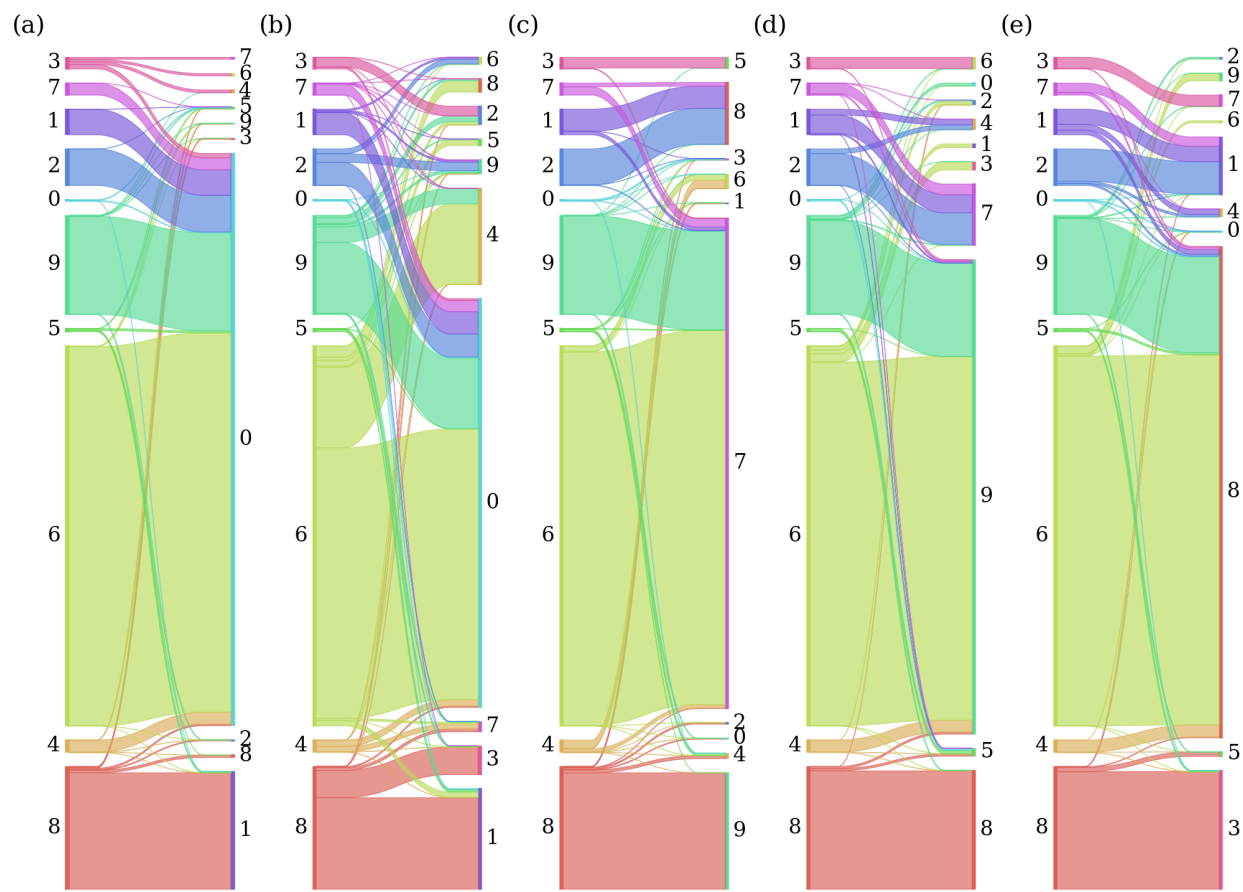

**Supplementary Figure 31:** The impact of employing alternative methods for macrostate construction is evaluated in comparison to the reference method SPIB for learning a 10-state model for Trp-cage. Each Sankey diagram illustrates the states obtained using SPIB (on the left) juxtaposed with states from alternative methods (on the right): (a) tICA-MPP model, (b) PCA-MPP model, (c) tICA-PCCA+ model, (d) PCA-PCCA+ model, and (e) VAMPnets model.

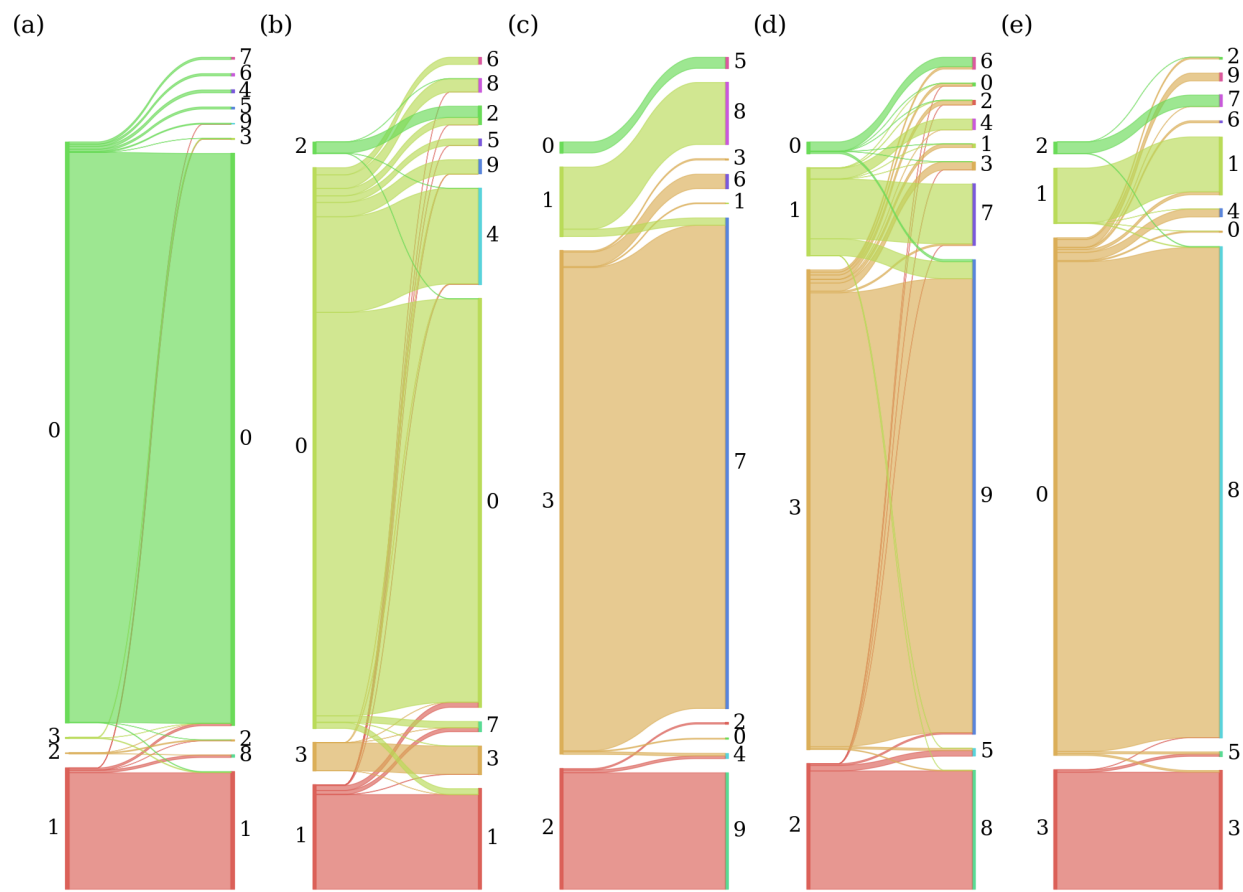

**Supplementary Figure 32:** Each Sankey diagram illustrates 4 states on the left juxtaposed with 10 states on the right for Trp-cage obtained using (a) tICA-MPP model, (b) PCA-MPP model, (c) tICA-PCCA+ model, (d) PCA-PCCA+ model, and (e) VAMPnets model.

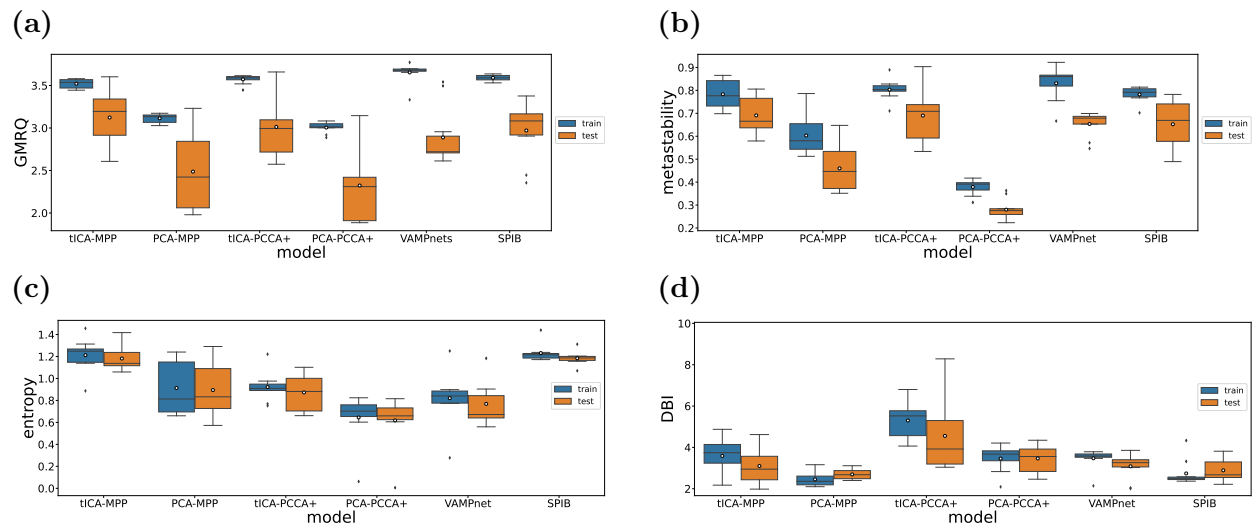

**Supplementary Figure 33:** HP35 quantitative results for 5-state model. The GMRQ scores are calculated using top 3 eigenvalues at a 100 ns lag time.

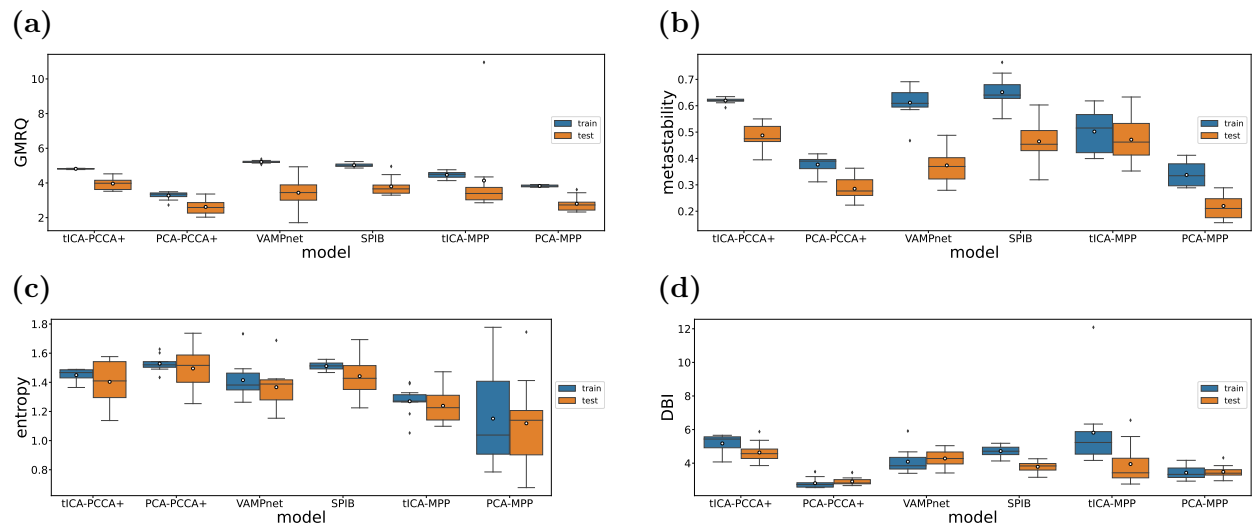

**Supplementary Figure 34:** HP35 quantitative results for 10-state model. The GMRQ scores are calculated using top 5 eigenvalues at a 100 ns lag time.

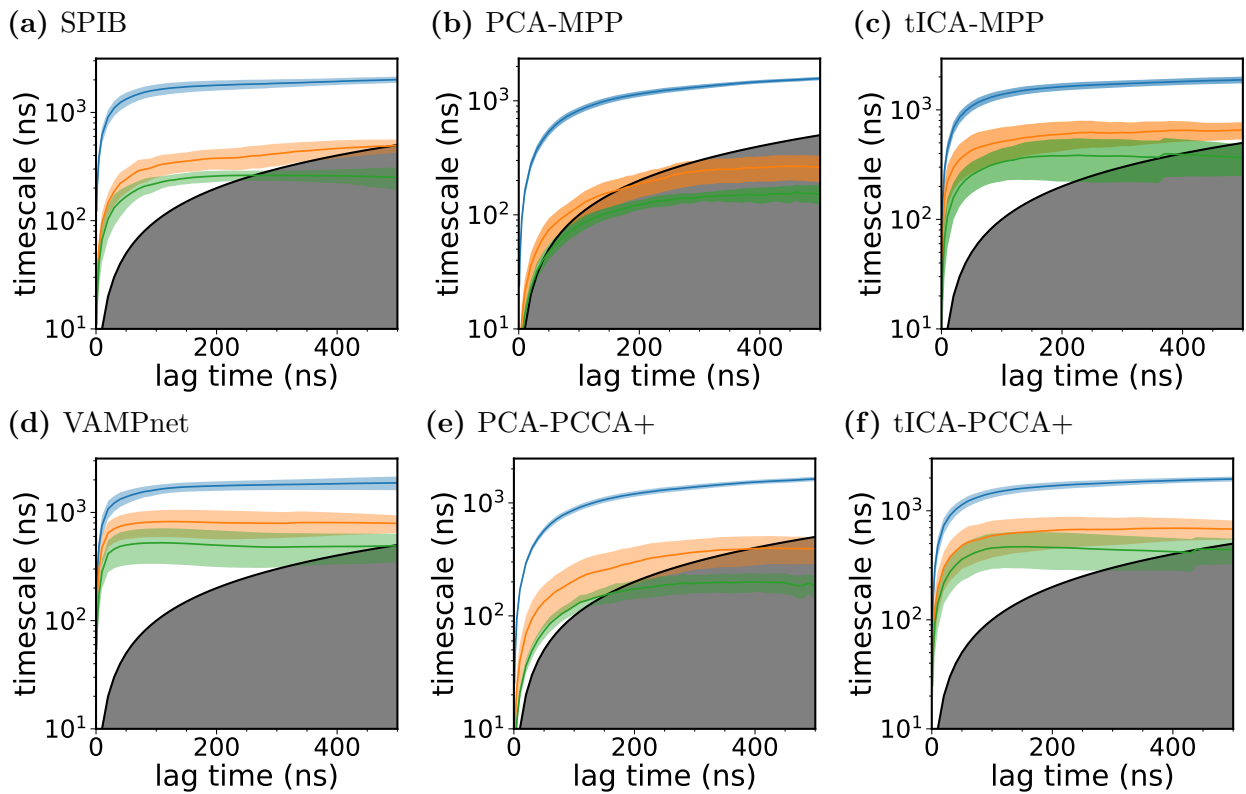

**Supplementary Figure 35:** Implied time scales as a function of lag time for 5-state MSMs of HP35. The shaded gray area represents the region where time scales become equal to or smaller than the lag time and can no longer be resolved. 95% confidence interval error bars are reported over 10 bootstrapping runs.

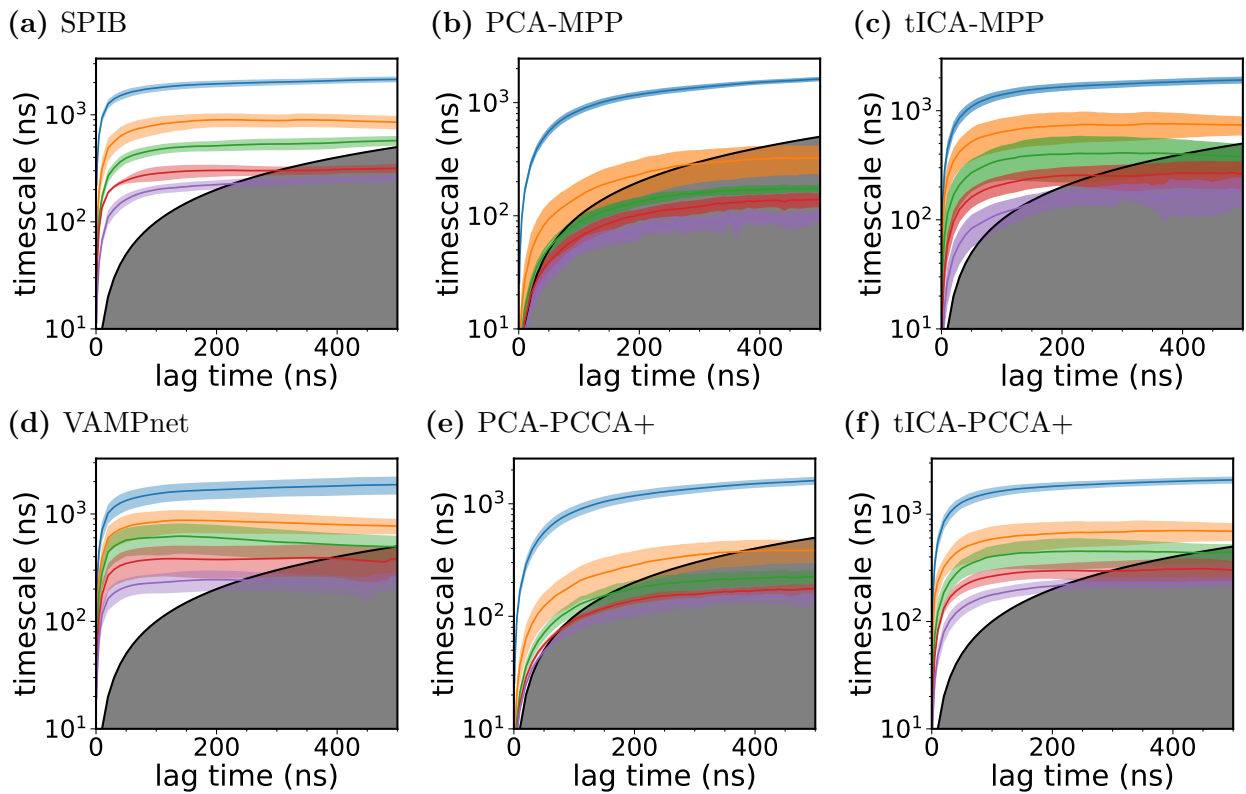

**Supplementary Figure 36:** Implied time scales as a function of lag time for 10-state MSMs of HP35. The shaded gray area represents the region where time scales become equal to or smaller than the lag time and can no longer be resolved. 95% confidence interval error bars are reported over 10 bootstrapping runs.

(a) 5-state

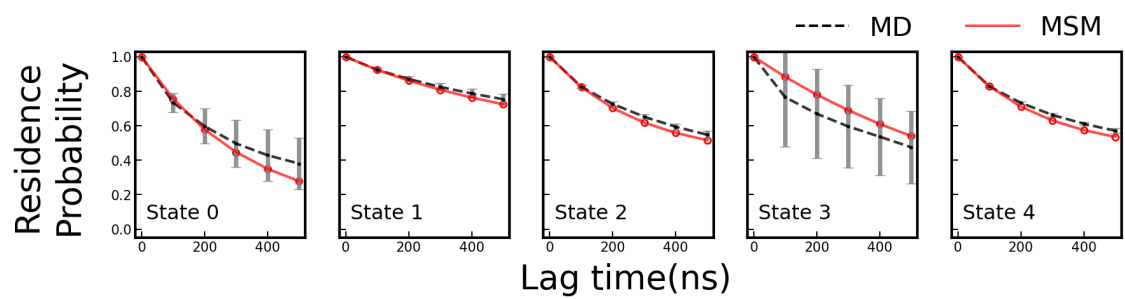

(b) 10-state

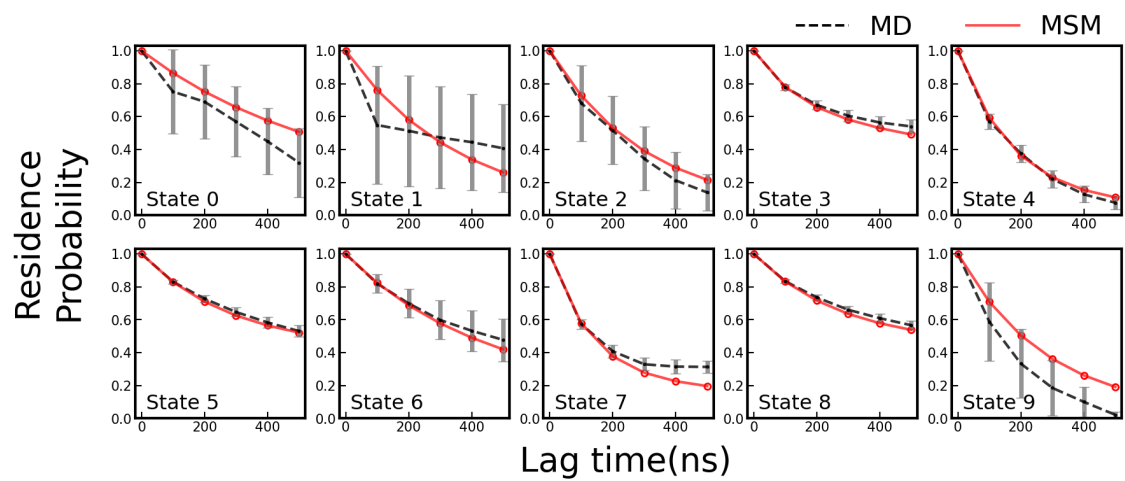

**Supplementary Figure 37:** The Chapman-Kolmogorov (CK) test utilizes residence probabilities for both the 5-macrostate (a) and 10-macrostate (b) MSMs constructed by SPIB for the HP35 folding system. The agreement between the residence probabilities predicted by 100ns SPIB-MSMs (solid red line) and those directly estimated from MD simulations (dashed black line) serves as validation for the MSMs. The error bar is estimated by bootstrapping MD trajectories 25 times with replacement for the 5-state model and 50 times with replacement for the 10-state model.

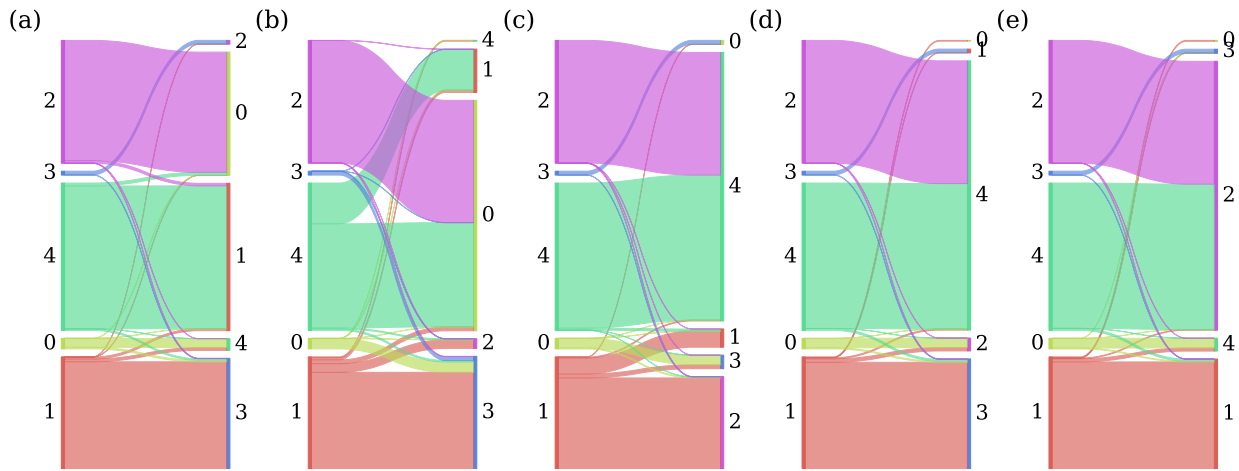

**Supplementary Figure 38:** For the HP35 system, the impact of employing alternative methods for macrostate construction is evaluated in comparison to the reference method SPIB for learning a 5-state model. Each Sankey diagram illustrates the states obtained using SPIB (on the left) juxtaposed with states from alternative methods (on the right): (a) tICA-MPP model, (b) PCA-MPP model, (c) tICA-PCCA+ model, (d) PCA-PCCA+ model, and (e) VAMPnets model.

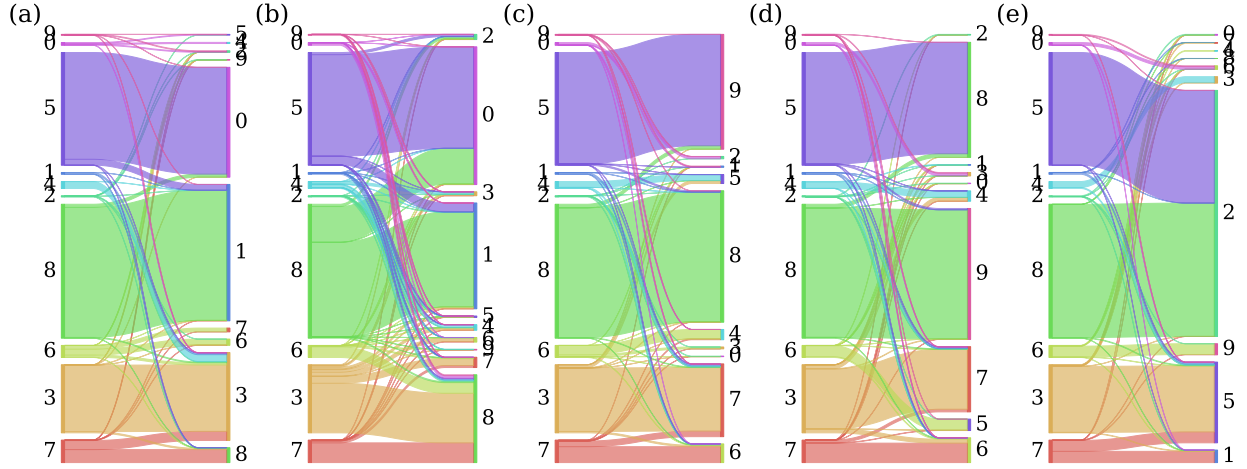

**Supplementary Figure 39:** For the HP35 system, the impact of employing alternative methods for macrostate construction is evaluated in comparison to the reference method SPIB for learning a 10-state model. Each Sankey diagram illustrates the states obtained using SPIB (on the left) juxtaposed with states from alternative methods (on the right): (a) tICA-MPP model, (b) PCA-MPP model, (c) tICA-PCCA+ model, (d) PCA-PCCA+ model, and (e) VAMPnets model.

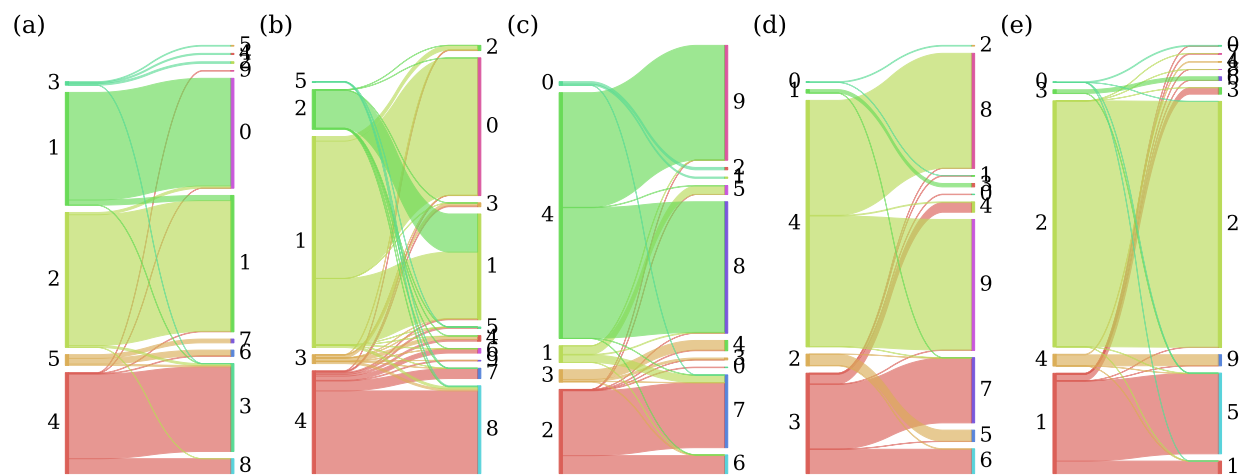

**Supplementary Figure 40:** Each Sankey diagram illustrates 5 states on the left juxtaposed with 10 states on the right for the HP35 system obtained using (a) tICA-MPP model, (b) PCA-MPP model, (c) tICA-PCCA+ model, (d) PCA-PCCA+ model, and (e) VAMPnets model.

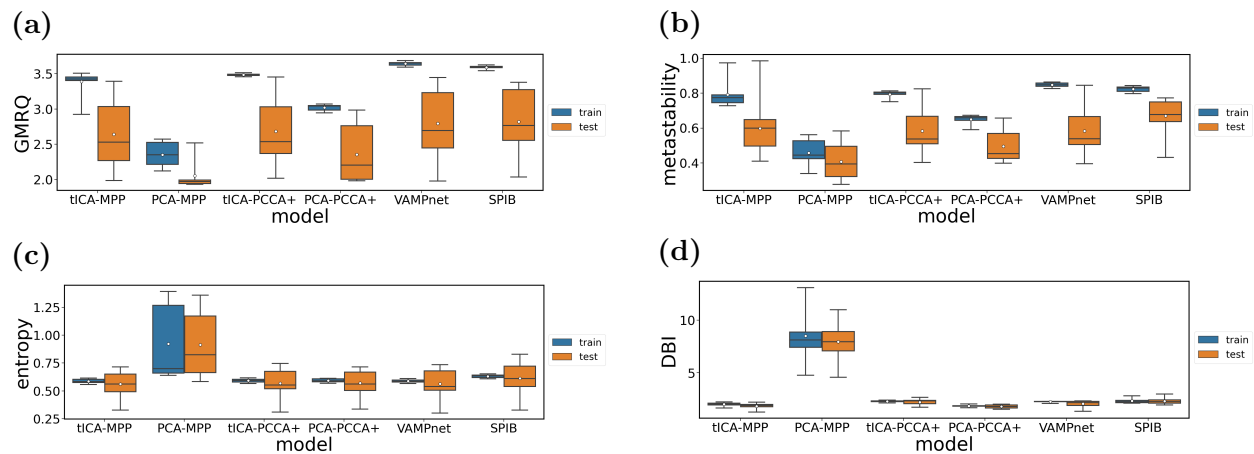

**Supplementary Figure 41:** WW-domain quantitative results for 5-state model. The GMQR scores are calculated using top 3 eigenvalues at a 100 ns lag time.

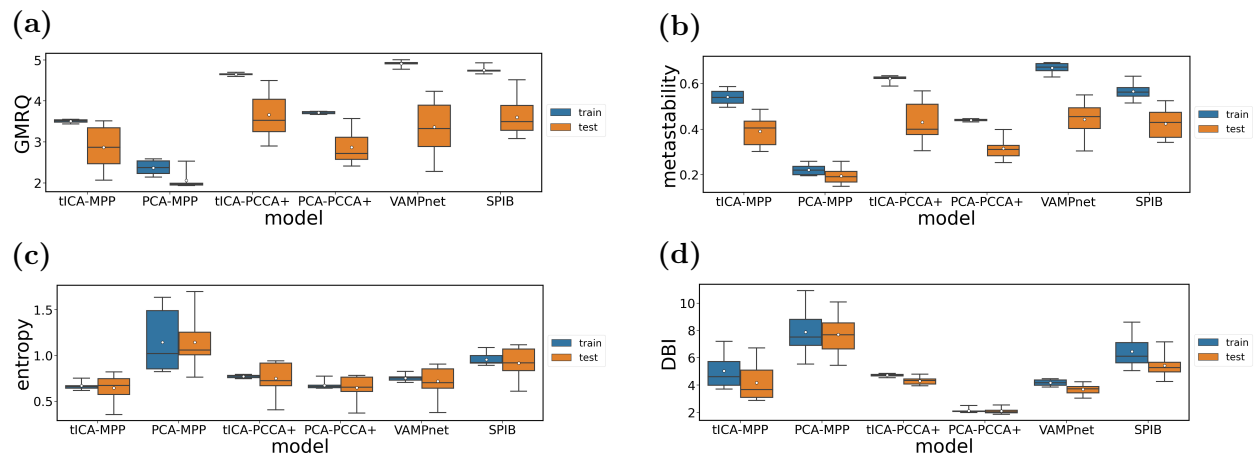

**Supplementary Figure 42:** WW-domain quantitative results for 10-state model. The GMRQ scores are calculated using top 5 eigenvalues at a 100 ns lag time.

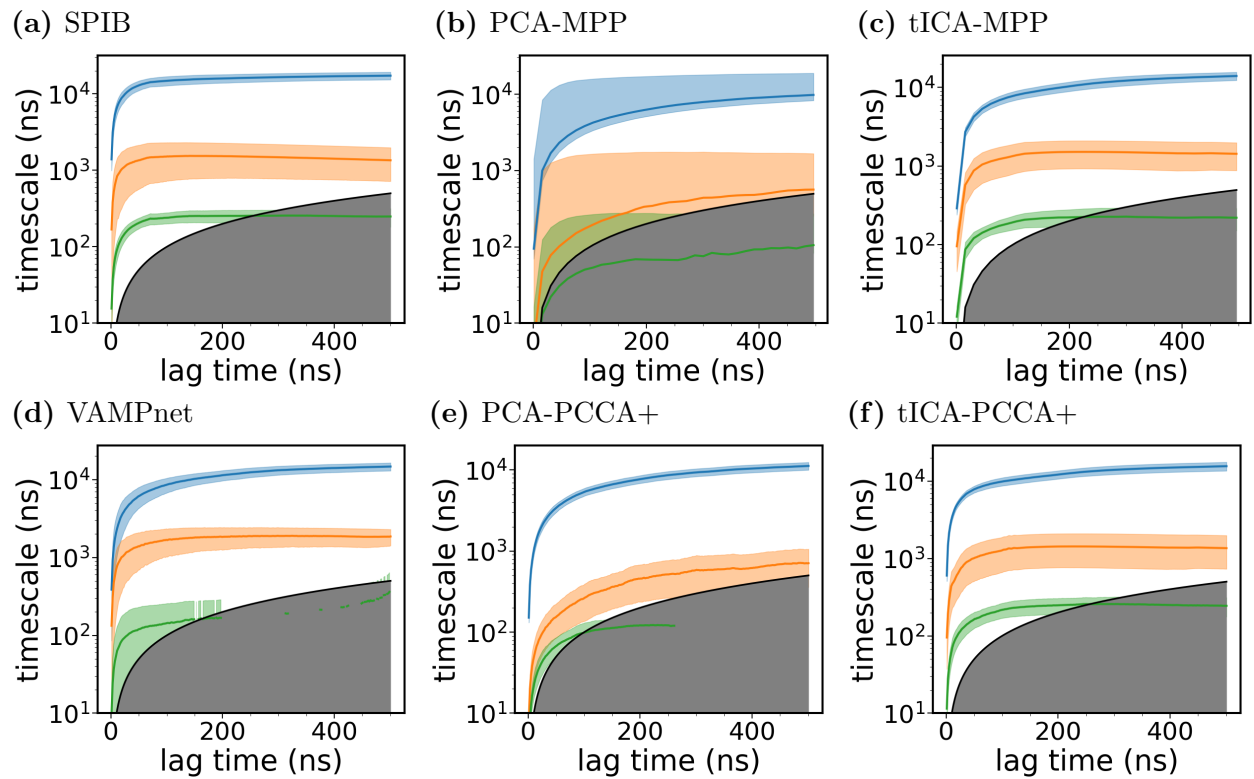

**Supplementary Figure 43:** Implied time scales as a function of lag time for the 5-state MSMs of WW-domain. The shaded gray area represents the region where time scales become equal to or smaller than the lag time and can no longer be resolved. 95% confidence interval error bars are reported over 10 bootstrapping runs.

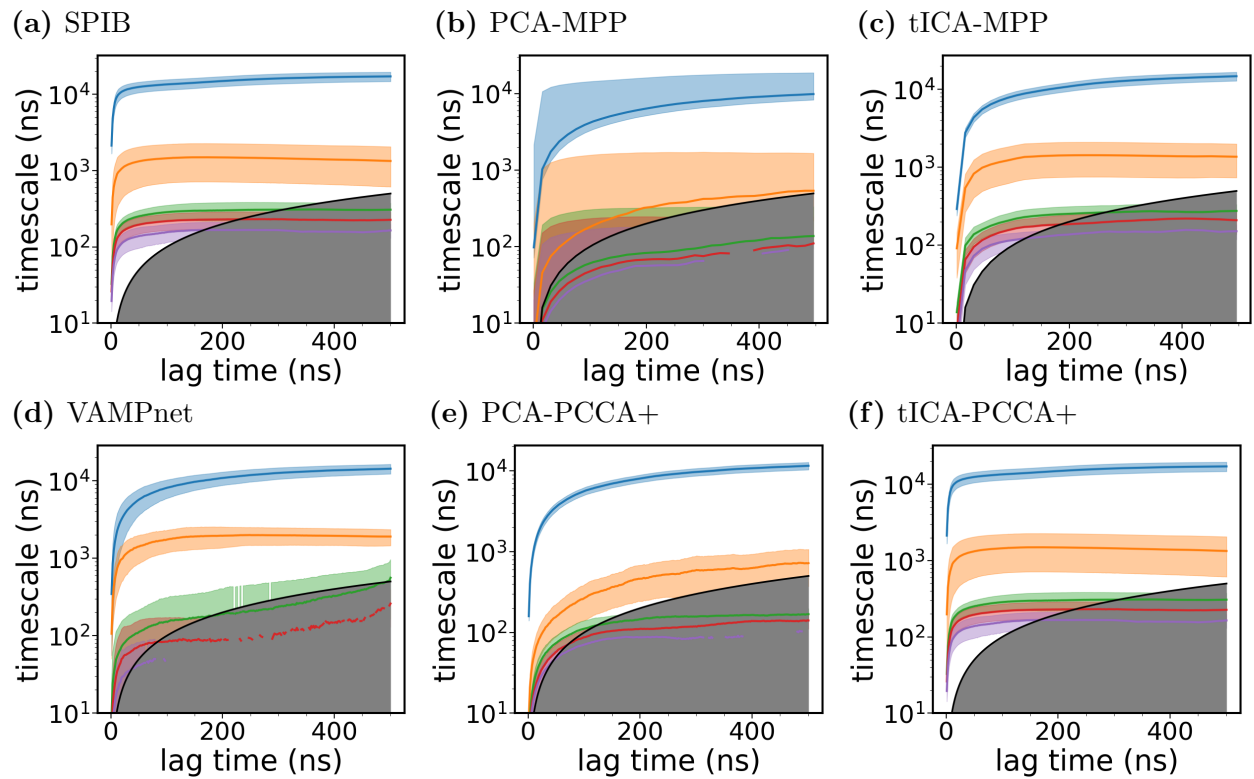

**Supplementary Figure 44:** Implied time scales as a function of lag time for the 10-state MSMs of WW-domain. The shaded gray area represents the region where time scales become equal to or smaller than the lag time and can no longer be resolved. 95% confidence interval error bars are reported over 10 bootstrapping runs.

(a) 5-state

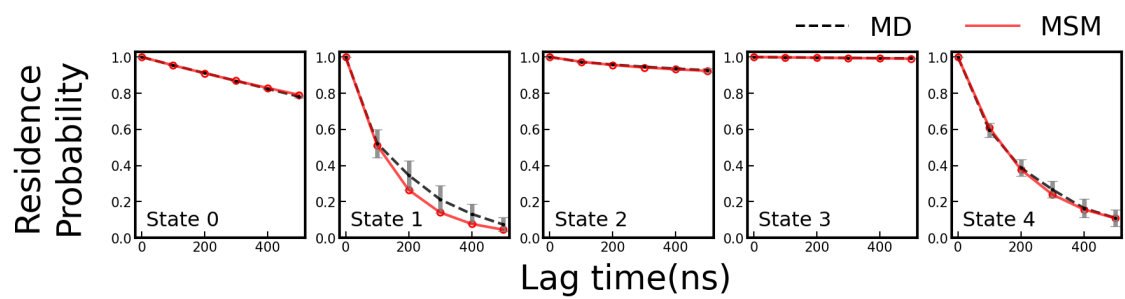

(b) 10-state

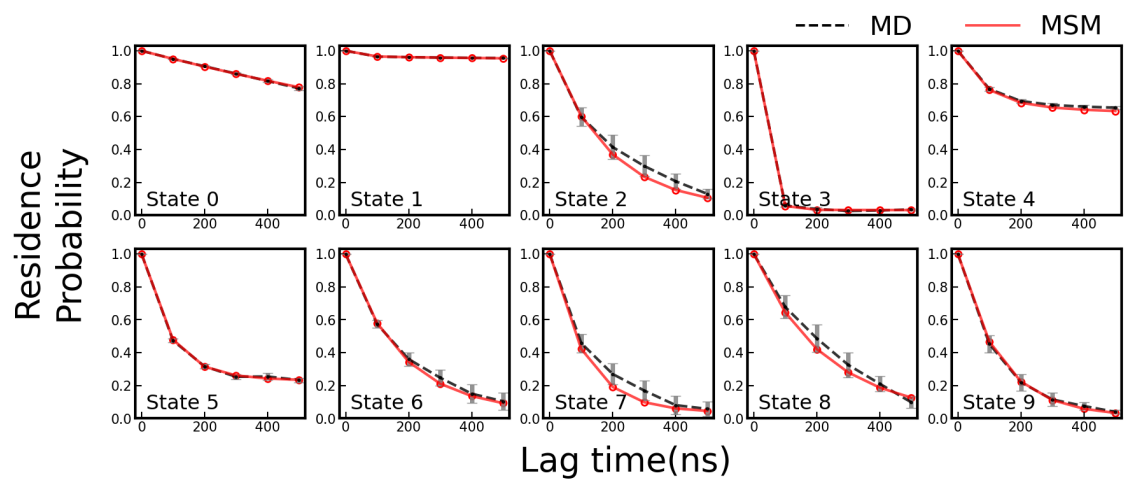

**Supplementary Figure 45:** The Chapman-Kolmogorov (CK) test utilizes residence probabilities for both the 5-macrostate (a) and 10-macrostate (b) MSMs constructed by SPIB for the WW-domain folding system. The agreement between the residence probabilities predicted by 100ns SPIB-MSMs (solid red line) and those directly estimated from MD simulations (dashed black line) serves as validation for the MSMs. The error bar is estimated by bootstrapping MD trajectories 50 times with replacement.

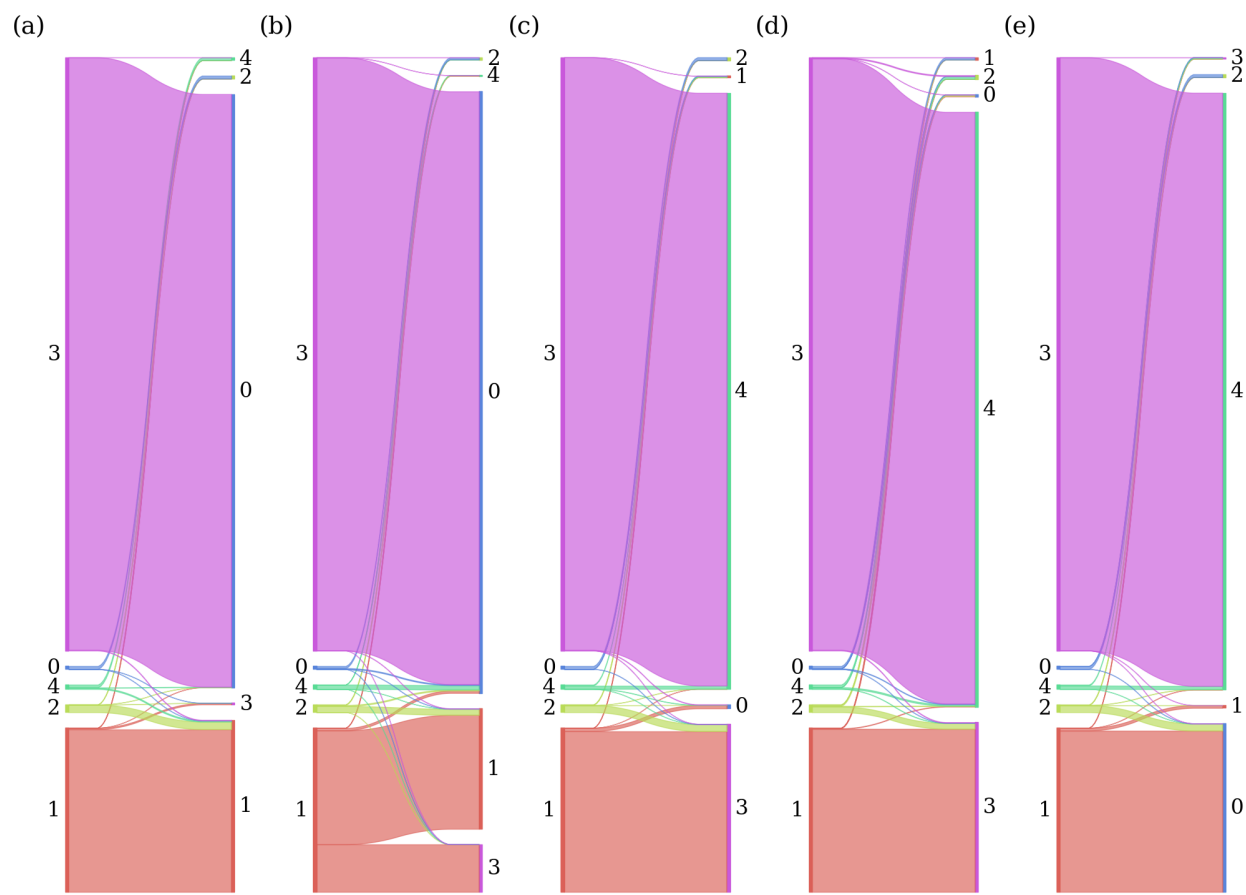

**Supplementary Figure 46:** For the WW-domain system, the impact of employing alternative methods for macrostate construction is evaluated in comparison to the reference method SPIB for learning a 5-state model. Each Sankey diagram illustrates the states obtained using SPIB (on the left) juxtaposed with states from alternative methods (on the right): (a) tICA-MPP model, (b) PCA-MPP model, (c) tICA-PCCA+ model, (d) PCA-PCCA+ model, and (e) VAMPnets model.

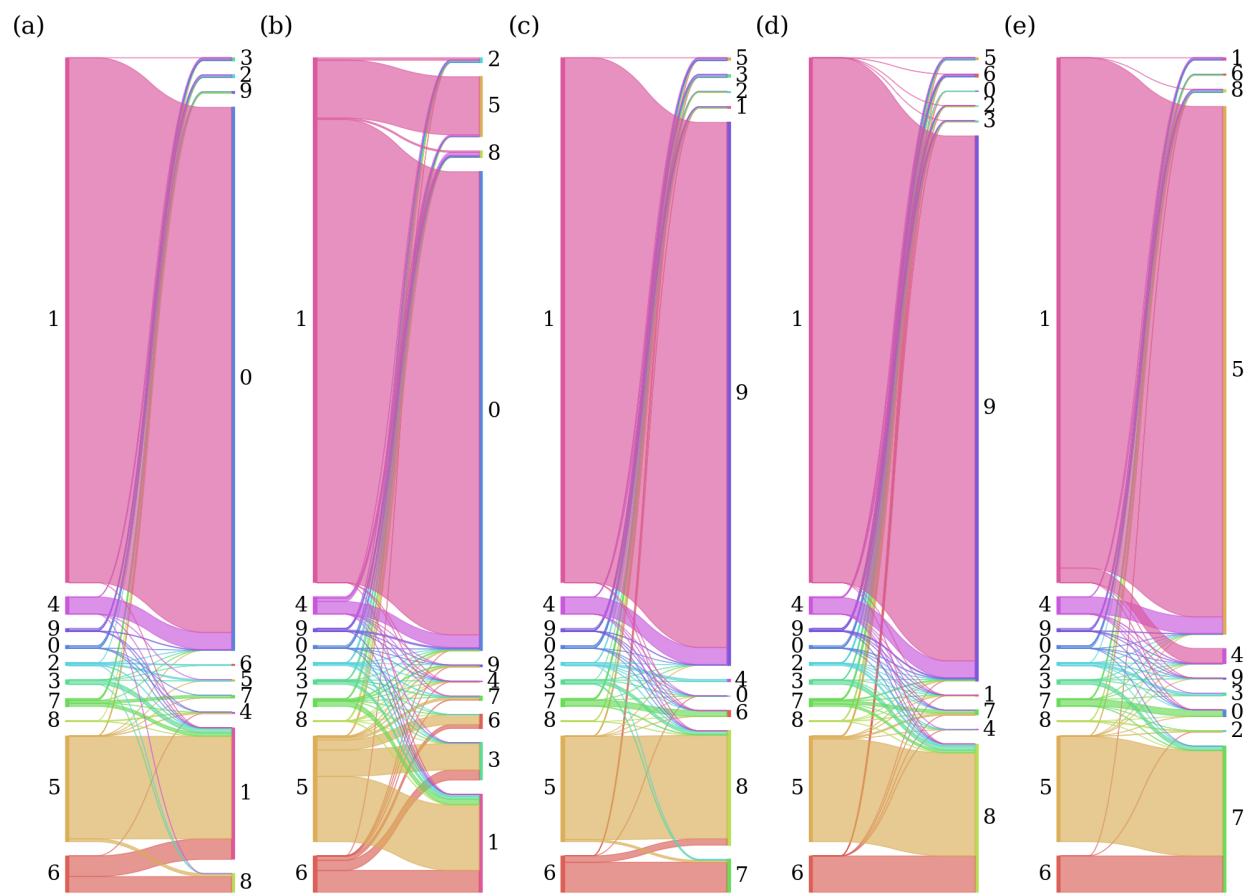

**Supplementary Figure 47:** For the WW-domain system, the impact of employing alternative methods for macrostate construction is evaluated in comparison to the reference method SPIB for learning a 10-state model. Each Sankey diagram illustrates the states obtained using SPIB (on the left) juxtaposed with states from alternative methods (on the right): (a) tICA-MPP model, (b) PCA-MPP model, (c) tICA-PCCA+ model, (d) PCA-PCCA+ model, and (e) VAMPnets model.

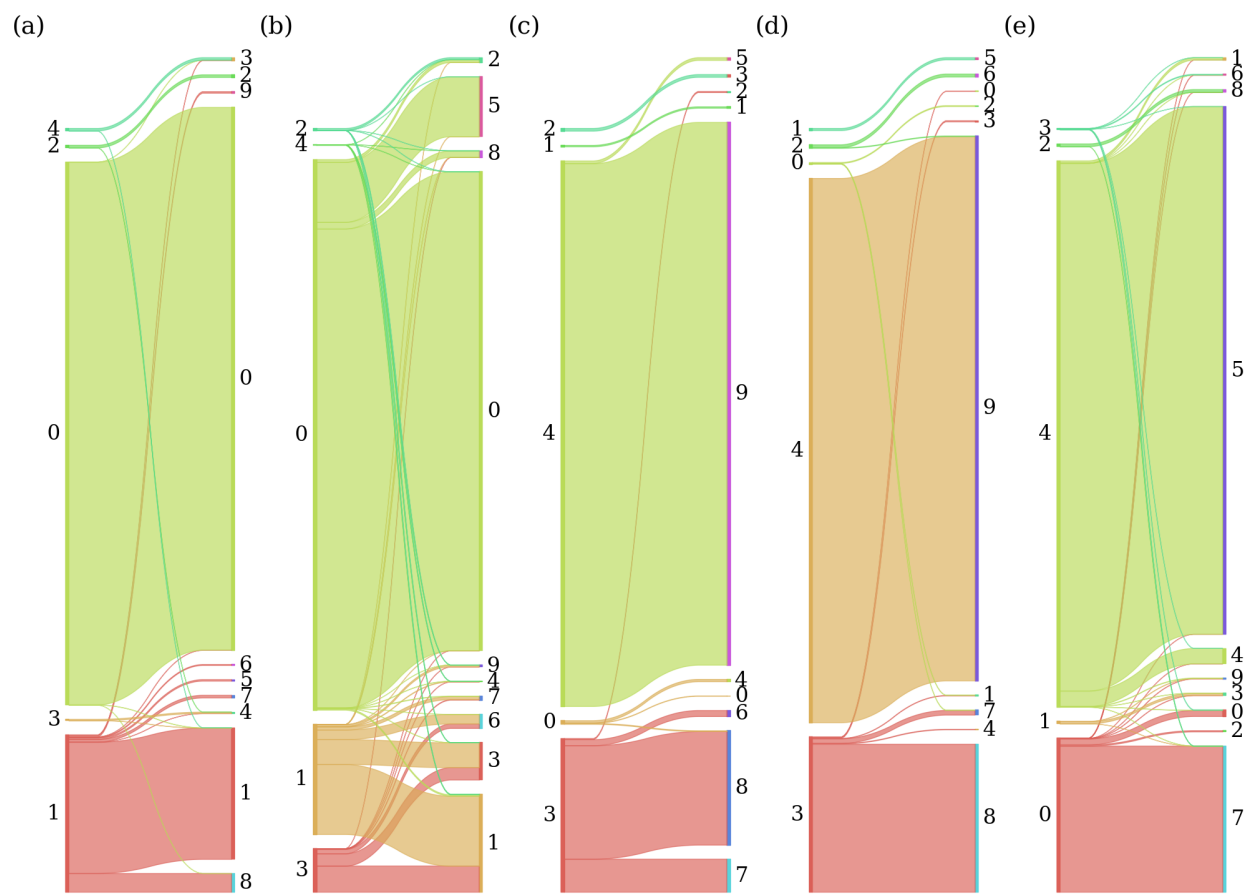

**Supplementary Figure 48:** Each Sankey diagram illustrates 5 states on the left juxtaposed with 10 states on the right for the WW-domain system obtained using (a) tICA-MPP model, (b) PCA-MPP model, (c) tICA-PCCA+ model, (d) PCA-PCCA+ model, and (e) VAMPnets model.
